# Supplementary material for: A Low-complexity Brain-computer Interface for High-complexity Robot Swarm Control
Source: arXiv:2205.14265 ancillary file (2022-05-27)
Supplement: Supplementary file 1 [file userstudy.pdf]

Consent Form

Georgia Institute of Technology - Consent Form

Title: Assessing Proficiency in Sorting a Heterogeneous, Geometric Lexicon  
Principal Investigator: Christopher Rozell, Ph. D.

I. Purpose: The purpose of this study is to assess human ability in sorting shapes according to a predefined ordering. This information will be utilized in the design of interfaces that use simple commands to control complex systems. We expect to enroll at least 150 individuals in this study.

II. Procedures: If you decide to participate in this study, we will ask you to look at pairs of shapes in various configurations and sort the shapes via computer mouse clicks according to an ordering that we will teach you in the study instructions. With your permission, we will record the time throughout the exercise as well as the shapes you select. The entire session will take approximately 1 hour.

III. Risks: In this study, you will not have any more risks than you would in a normal day of life. The risks involved are no greater than those involved in daily computer based activities such as typing on the keyboard or moving a computer mouse.

IV. Benefits: You may or may not benefit from this study directly. We hope that participation in this project will lead to methods for controlling complex systems with simple commands.

V. Compensation and Costs to You: You will be compensated \$8 for your time and effort, contingent on completion of all tasks in this study. In addition, you will be awarded a bonus of \$4 if you answer more than 95% of all questions correctly. U.S. Tax Law requires a mandatory withholding of 30% for nonresident alien payments of any type. Your address and citizenship/visa status may be collected for compensation purposes only. This information will be shared only with the Georgia Tech department that issues compensation, if any, for your participation. There are no financial obligations for you to participate.

VI. Confidentiality: We will keep your records private to the extent allowed by law. To protect your privacy, records will be kept under a code number rather than by name. Your name and any facts that might point to your identity will not appear when we present this study or publish its findings. The findings will be summarized and reported in group form. You will not be identified personally. Information may also be shared with those who make sure the study is done correctly (Georgia Institute of Technology Institutional Review Board, the Office for Human Research Protection (OHRP)).

VII. In Case of Injury/Harm: If you are injured as a result of being in this study, please contact Dr. C. Rozell at telephone (404) 385-7671. Neither the Principal Investigator nor the Georgia Institute of Technology has made provision for payment of costs associated with any injury resulting from participation in this study.

VIII. Subject Rights: Participation in this study is voluntary. You do not have to be in this study. If you change your mind, you have the right to withdraw at any time. Any new information that may make you change your mind about being in this study will be given to you.

IX. Questions about the Study or Your Rights as a Research Subject: If you have any questions about the study, you may contact Dr. C. Rozell at telephone (404) 385-7671. If you have any questions about your rights as a research subject, you may contact Ms. Melanie Clark at (404) 894-6942.

**By submitting this HIT, it means that you have read, or have had read to you, the information contained in this letter and would like to be a volunteer in this research study. Thank you.**

Instructions

When we're kids, we're taught how to put words in alphabetical order. For example, "cash" comes before "taxi" and "star" comes before "step." If we give you a *test* word and a *reference* word, how do you know if the *test* word comes **before** or **after** the *reference* word in the dictionary? You start by ignoring letters that are the same and finding the first letter position that's different. If the *test* letter is **before** the *reference* letter in the alphabet, then the *test* word is **before** the *reference* word in the dictionary. If the *test* letter is **after** the *reference* letter in the alphabet, then the *test* word is **after** the *reference* word in the dictionary. To illustrate:

Example) test: "sand"      reference: "same"

|            |      |      |       |                |
|------------|------|------|-------|----------------|
| test       | s    | a    | n     | d              |
| reference  | s    | a    | m     | e              |
| comparison | same | same | after | doesn't matter |

The first two letter positions ("s" and "a") are the same, so we move on to the third letter position. Because "n" comes after "m" in the alphabet, the *test* word comes **after** the *reference* word in the dictionary. The last letter position doesn't matter.

In this HIT we will teach you how to alphabetize shapes using the same approach. After some instruction, you will be given a test shape (red, dashed edges) and asked if it comes **before** or **after** a reference shape (blue, solid edges), just like we did for words! The only difference is that shapes will be treated as four-letter words where we will use visual features (location, number of sides, size) for each letter position. Here is a table to help us out:

|                              | 1 <sup>st</sup> letter position<br>side-to-side location | 2 <sup>nd</sup> letter position<br>up-down location | 3 <sup>rd</sup> letter position<br>number of sides | 4 <sup>th</sup> letter position<br>size |
|------------------------------|----------------------------------------------------------|-----------------------------------------------------|----------------------------------------------------|-----------------------------------------|
| test <b>after</b> reference  | test is <b>right</b>                                     | test is <b>above</b>                                | test has <b>more sides</b>                         | test is <b>larger</b>                   |
| test <b>before</b> reference | test is <b>left</b>                                      | test is <b>below</b>                                | test has <b>less sides</b>                         | test is <b>smaller</b>                  |

Start at the first column of the table, showing that the first letter position is the side-to-side location (of the center) of the shape. If the *test* shape is to the **left** of the *reference* shape, then you say the *test* shape comes **before**. If it's to the **right** of the *reference*, you say **after**.

If they're at the **same** side-to-side location, go to the second column in the table showing that the second letter position is the up-down location (of the center) of the shape. If the test is **below** the reference, select **before**. If it's **above** the reference, select **after**.

If they are at the **same** up-down location, go to the third column in the table showing that the third letter position is the number of sides (e.g., triangle=3, diamond=4, etc.) of the shape. If the *test* has **less sides** than the *reference*, select **before**. If it has **more sides** than the *reference*, select **after**.

If they have the **same** number of sides, go to the fourth column in the table showing that the last letter position is the size of the shape. If the *test* is **smaller** than the *reference*, select **before**. If it is **larger** than the *reference*, select **after**.

We simplified this table to a "cheat sheet" which you can use during the HIT:

|        | 1 <sup>st</sup> letter position<br>side-to-side location | 2 <sup>nd</sup> letter position<br>up-down location | 3 <sup>rd</sup> letter position<br>number of sides | 4 <sup>th</sup> letter position<br>size |
|--------|----------------------------------------------------------|-----------------------------------------------------|----------------------------------------------------|-----------------------------------------|
| after  | right                                                    | above                                               | more sides                                         | larger                                  |
| before | left                                                     | below                                               | less sides                                         | smaller                                 |

Let's use this cheat sheet to solve a few examples, where the *test* shape has red dashed edges, and the *reference* shape has blue solid edges:

|        | 1 <sup>st</sup> letter position<br>side-to-side location | 2 <sup>nd</sup> letter position<br>up-down location | 3 <sup>rd</sup> letter position<br>number of sides | 4 <sup>th</sup> letter position<br>size |
|--------|----------------------------------------------------------|-----------------------------------------------------|----------------------------------------------------|-----------------------------------------|
| after  | right                                                    | above                                               | more sides                                         | larger                                  |
| before | left                                                     | below                                               | less sides                                         | smaller                                 |

The *test* shape is to the **left** of the *reference* shape, so we say it comes **before**. We're done, so nothing else about the shapes matters!

|        | 1 <sup>st</sup> letter position<br>side-to-side location | 2 <sup>nd</sup> letter position<br>up-down location | 3 <sup>rd</sup> letter position<br>number of sides | 4 <sup>th</sup> letter position<br>size |
|--------|----------------------------------------------------------|-----------------------------------------------------|----------------------------------------------------|-----------------------------------------|
| after  | right                                                    | above                                               | more sides                                         | larger                                  |
| before | left                                                     | below                                               | less sides                                         | smaller                                 |

The *test* shape is to the **right** of the *reference* shape, so we say it comes **after**. We're done, so nothing else about the shapes matters!

|        | 1 <sup>st</sup> letter position<br>side-to-side location | 2 <sup>nd</sup> letter position<br>up-down location | 3 <sup>rd</sup> letter position<br>number of sides | 4 <sup>th</sup> letter position<br>size |
|--------|----------------------------------------------------------|-----------------------------------------------------|----------------------------------------------------|-----------------------------------------|
| after  | right                                                    | above                                               | more sides                                         | larger                                  |
| before | left                                                     | below                                               | less sides                                         | smaller                                 |

This time, the two shapes are at the same side-to-side location. Looking at up-down location, since the *test* shape is **below** the *reference* shape we say it comes **before**. We're done, so nothing else about the shapes matters!

|        | 1 <sup>st</sup> letter position<br>side-to-side location | 2 <sup>nd</sup> letter position<br>up-down location | 3 <sup>rd</sup> letter position<br>number of sides | 4 <sup>th</sup> letter position<br>size |
|--------|----------------------------------------------------------|-----------------------------------------------------|----------------------------------------------------|-----------------------------------------|
| after  | right                                                    | above                                               | more sides                                         | larger                                  |
| before | left                                                     | below                                               | less sides                                         | smaller                                 |

Now, the two shapes are at the same side-to-side location and the same up-down location. Looking at the number of sides, the *test* shape has **more sides** than the *reference* shape so we say it comes **after**. We're done, so the size of the shapes doesn't matter!

|        | 1 <sup>st</sup> letter position<br>side-to-side location | 2 <sup>nd</sup> letter position<br>up-down location | 3 <sup>rd</sup> letter position<br>number of sides | 4 <sup>th</sup> letter position<br>size |
|--------|----------------------------------------------------------|-----------------------------------------------------|----------------------------------------------------|-----------------------------------------|
| after  | right                                                    | above                                               | more sides                                         | larger                                  |
| before | left                                                     | below                                               | less sides                                         | smaller                                 |

In this last example, the two shapes are at the same side-to-side location, the same up-down location, and have the same number of sides. Looking at the size of each shape, the *test* shape is **smaller** than the *reference* shape so we say it comes **before**.

Now that you know how to "alphabetize" shapes, you'll do it for 150 pairs of *test* and *reference* shapes. Each pair will have the cheat sheet that you can use to remember the four letter positions and how to order them.

If you answer **ALL** questions in the HIT, you will be approved and paid **\$8.00**. Note we can detect if you simply select random answers in order to finish the HIT quickly without making a good faith effort. In this case your HIT will be rejected and you won't get paid. Incomplete HITs cannot be accepted, so make sure not to accidentally press "Enter" or the submit button during the task until you've marked each answer. In addition, you will be awarded a bonus of **\$4.00** if your work is approved and you answer more than **95%** of all questions correctly, so do your best work! **Only one "Sorting shapes using learned rules" HIT per worker (i.e. no repeats)**. Good luck!



\*\*\*After you have completed **EVERY** question in this HIT, click the submit button below. Note that incomplete HITs will **NOT** be approved and can **NOT** be resubmitted\*\*\*

1. For the image below, select whether the test shape (red dashed edges) comes after or before the reference shape (blue solid edges), as defined in the instructions above.

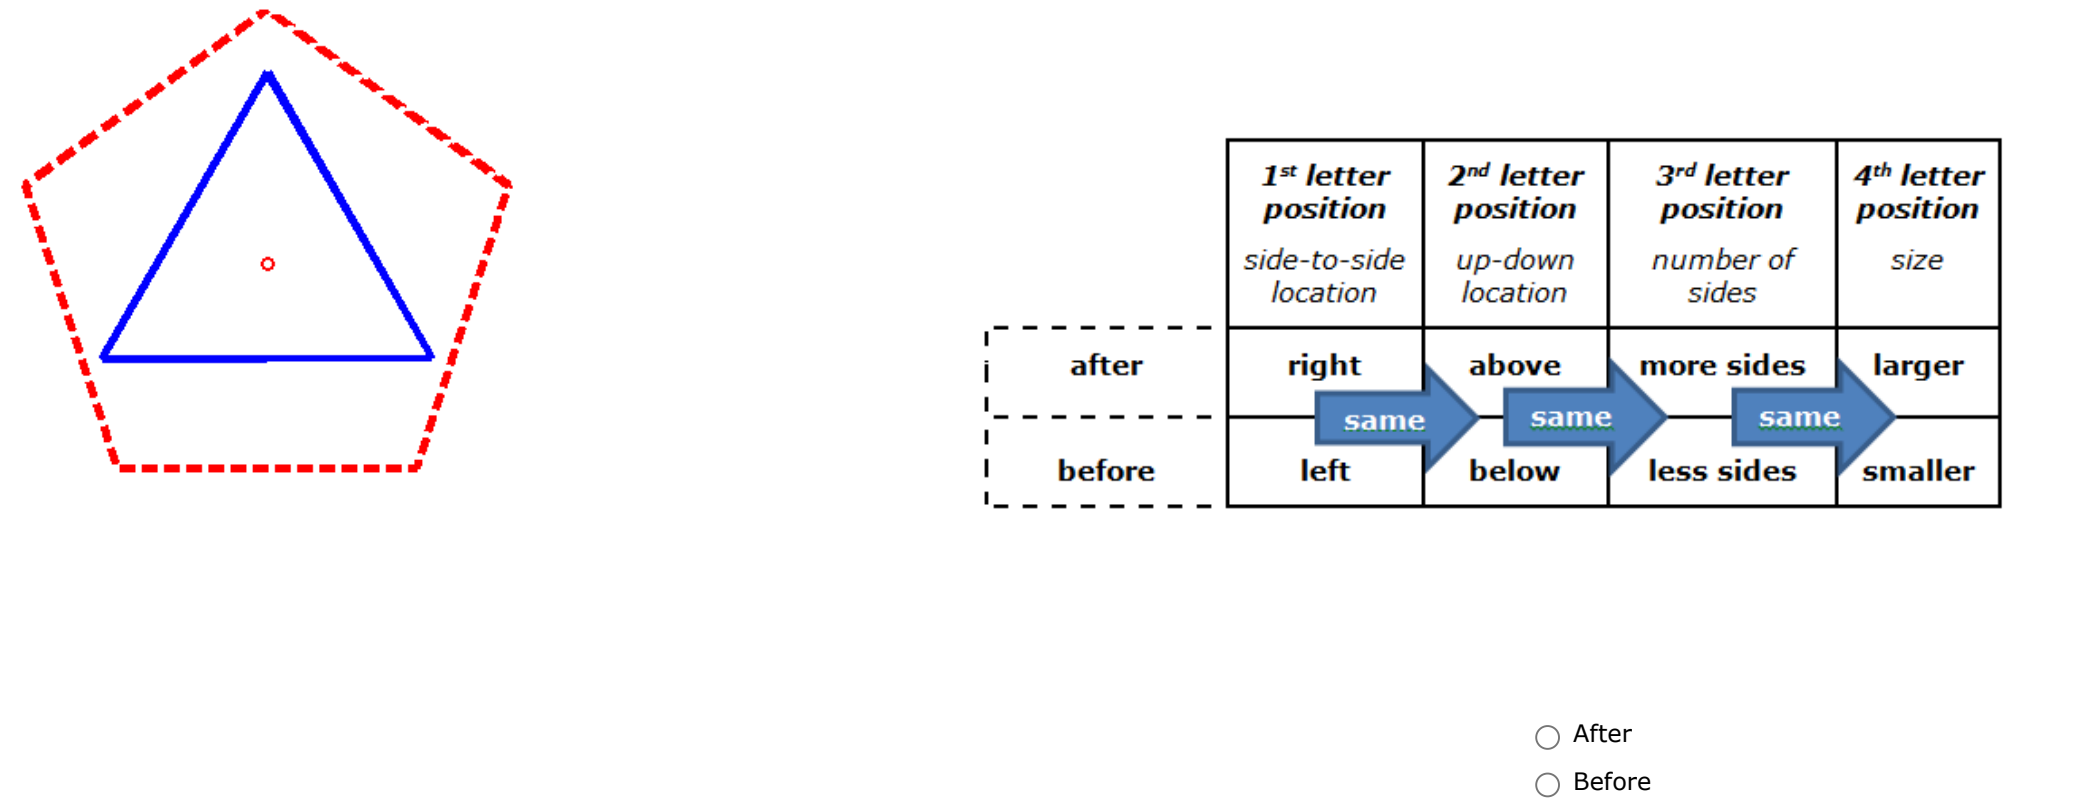

|        | 1 <sup>st</sup> letter<br>position<br>side-to-side<br>location | 2 <sup>nd</sup> letter<br>position<br>up-down<br>location | 3 <sup>rd</sup> letter<br>position<br>number of<br>sides | 4 <sup>th</sup> letter<br>position<br>size |
|--------|----------------------------------------------------------------|-----------------------------------------------------------|----------------------------------------------------------|--------------------------------------------|
| after  | right                                                          | above                                                     | more sides                                               | larger                                     |
| before | left                                                           | below                                                     | less sides                                               | smaller                                    |

☐ After  
☐ Before

2. For the image below, select whether the test shape (red dashed edges) comes after or before the reference shape (blue solid edges), as defined in the instructions above.

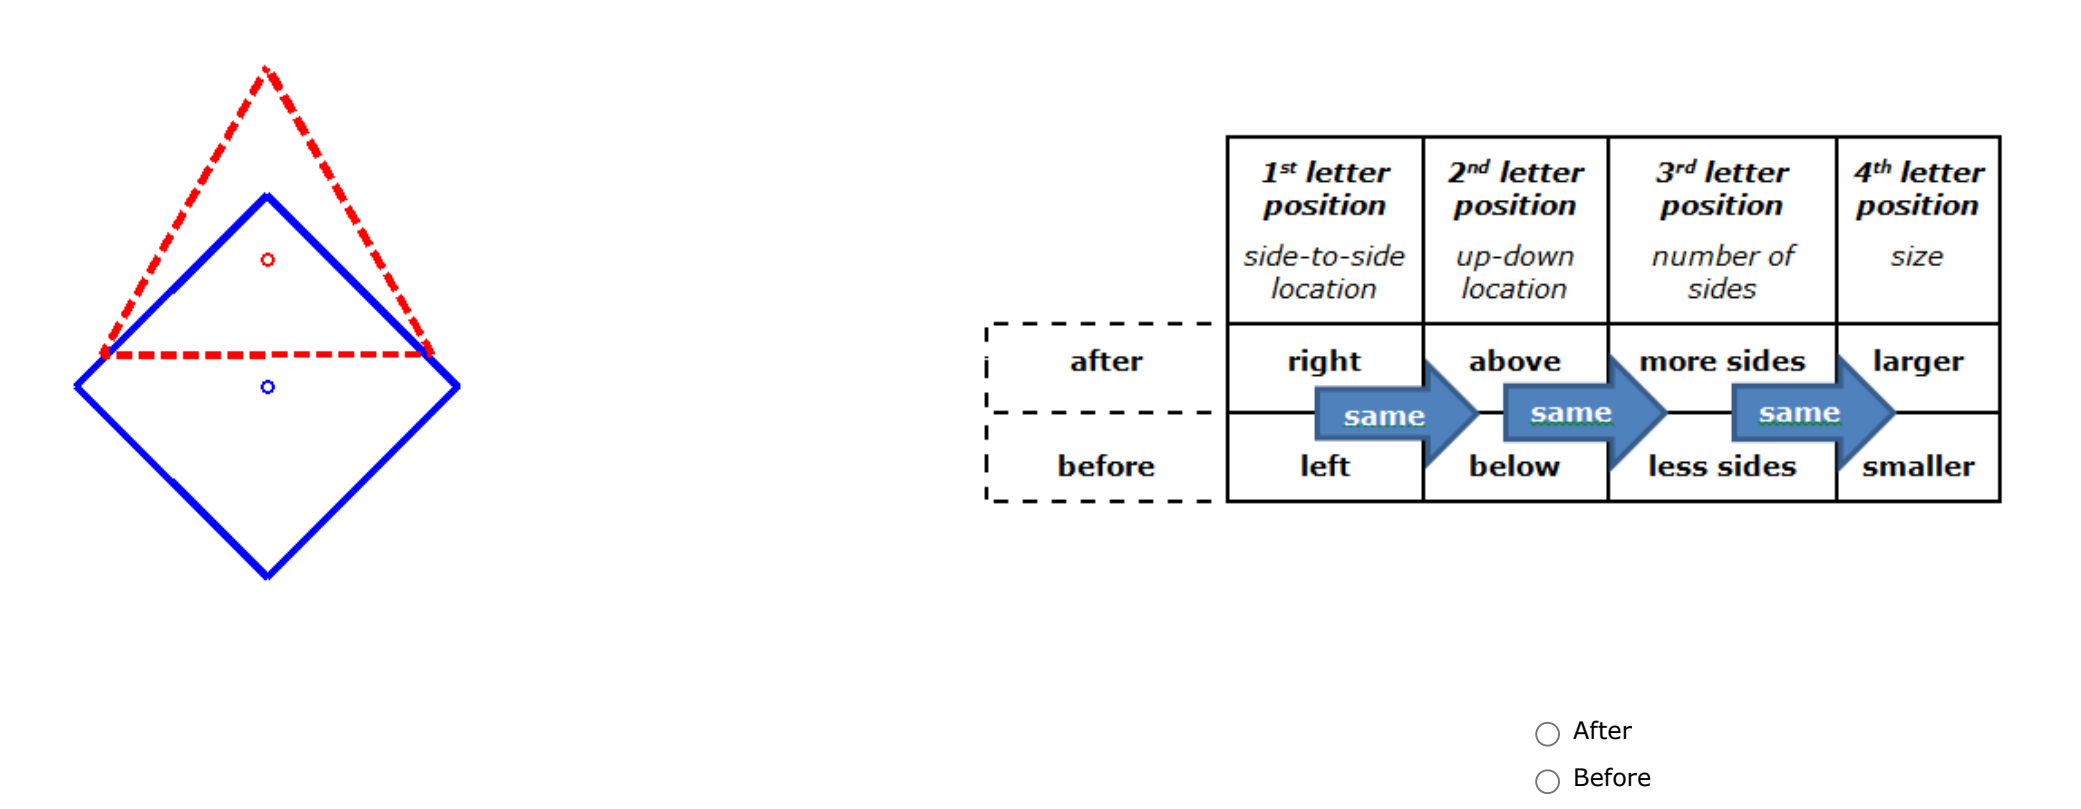

|        | 1 <sup>st</sup> letter<br>position<br>side-to-side<br>location | 2 <sup>nd</sup> letter<br>position<br>up-down<br>location | 3 <sup>rd</sup> letter<br>position<br>number of<br>sides | 4 <sup>th</sup> letter<br>position<br>size |
|--------|----------------------------------------------------------------|-----------------------------------------------------------|----------------------------------------------------------|--------------------------------------------|
| after  | right                                                          | above                                                     | more sides                                               | larger                                     |
| before | left                                                           | below                                                     | less sides                                               | smaller                                    |

☐ After  
☐ Before

3. For the image below, select whether the test shape (red dashed edges) comes after or before the reference shape (blue solid edges), as defined in the instructions above.

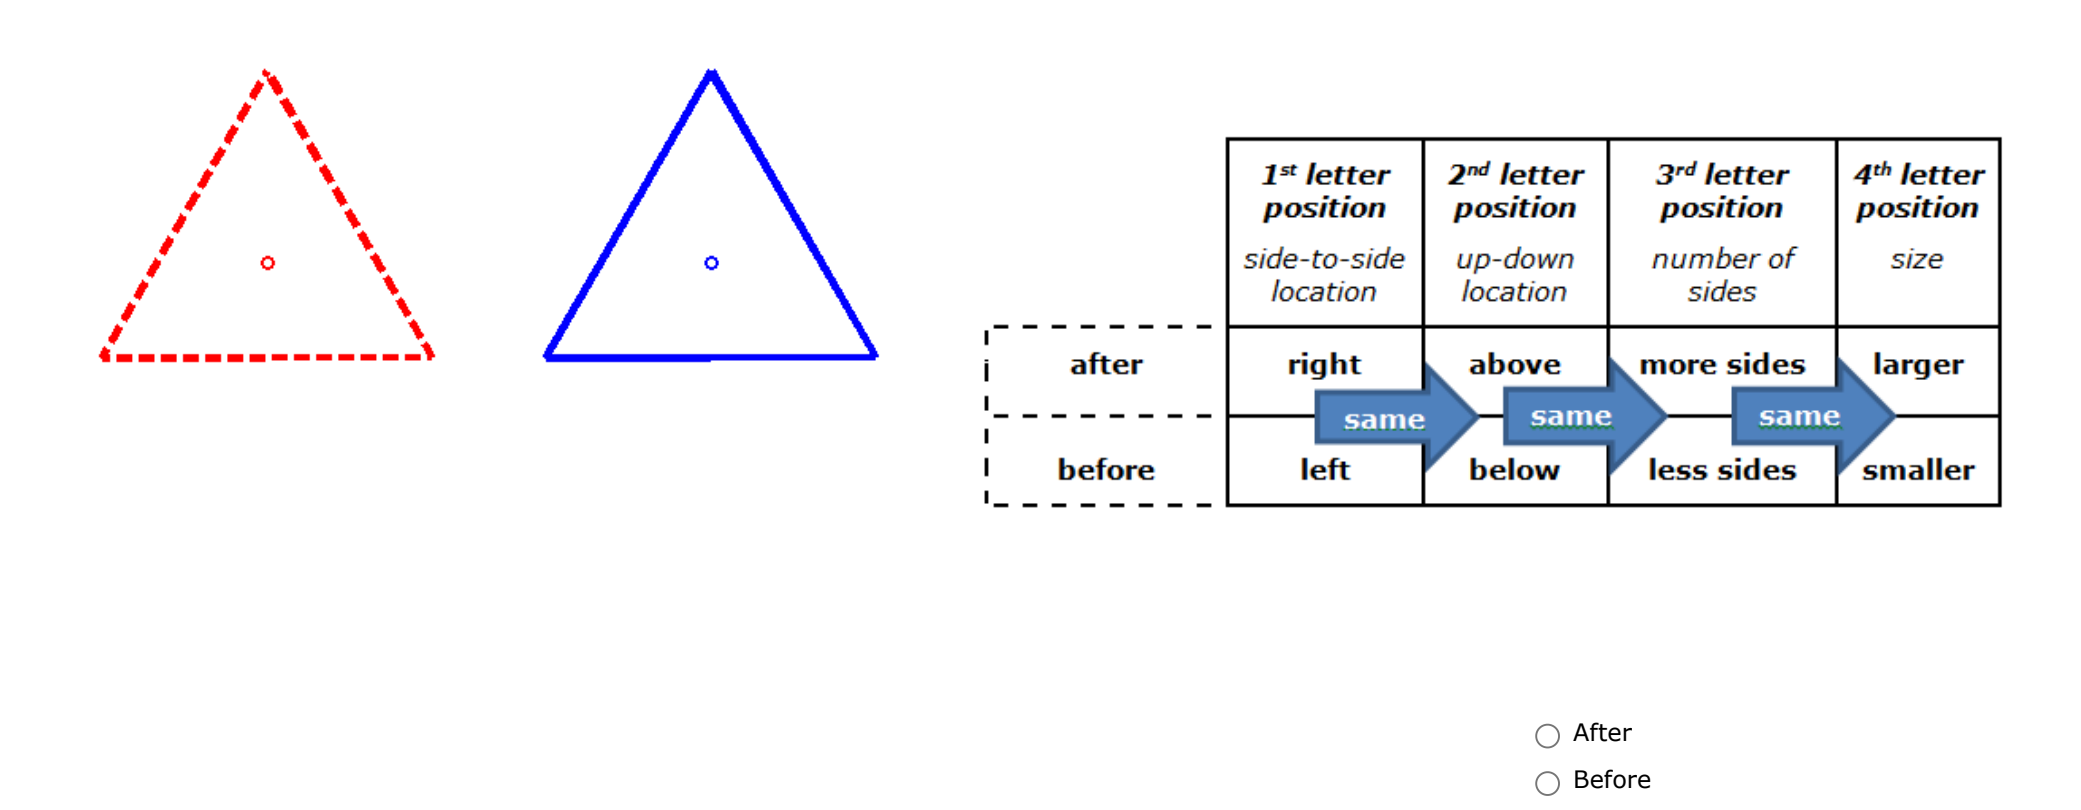

|        | 1 <sup>st</sup> letter<br>position<br>side-to-side<br>location | 2 <sup>nd</sup> letter<br>position<br>up-down<br>location | 3 <sup>rd</sup> letter<br>position<br>number of<br>sides | 4 <sup>th</sup> letter<br>position<br>size |
|--------|----------------------------------------------------------------|-----------------------------------------------------------|----------------------------------------------------------|--------------------------------------------|
| after  | right                                                          | above                                                     | more sides                                               | larger                                     |
| before | left                                                           | below                                                     | less sides                                               | smaller                                    |

☐ After  
☐ Before

4. For the image below, select whether the test shape (red dashed edges) comes after or before the reference shape (blue solid edges), as defined in the instructions above.

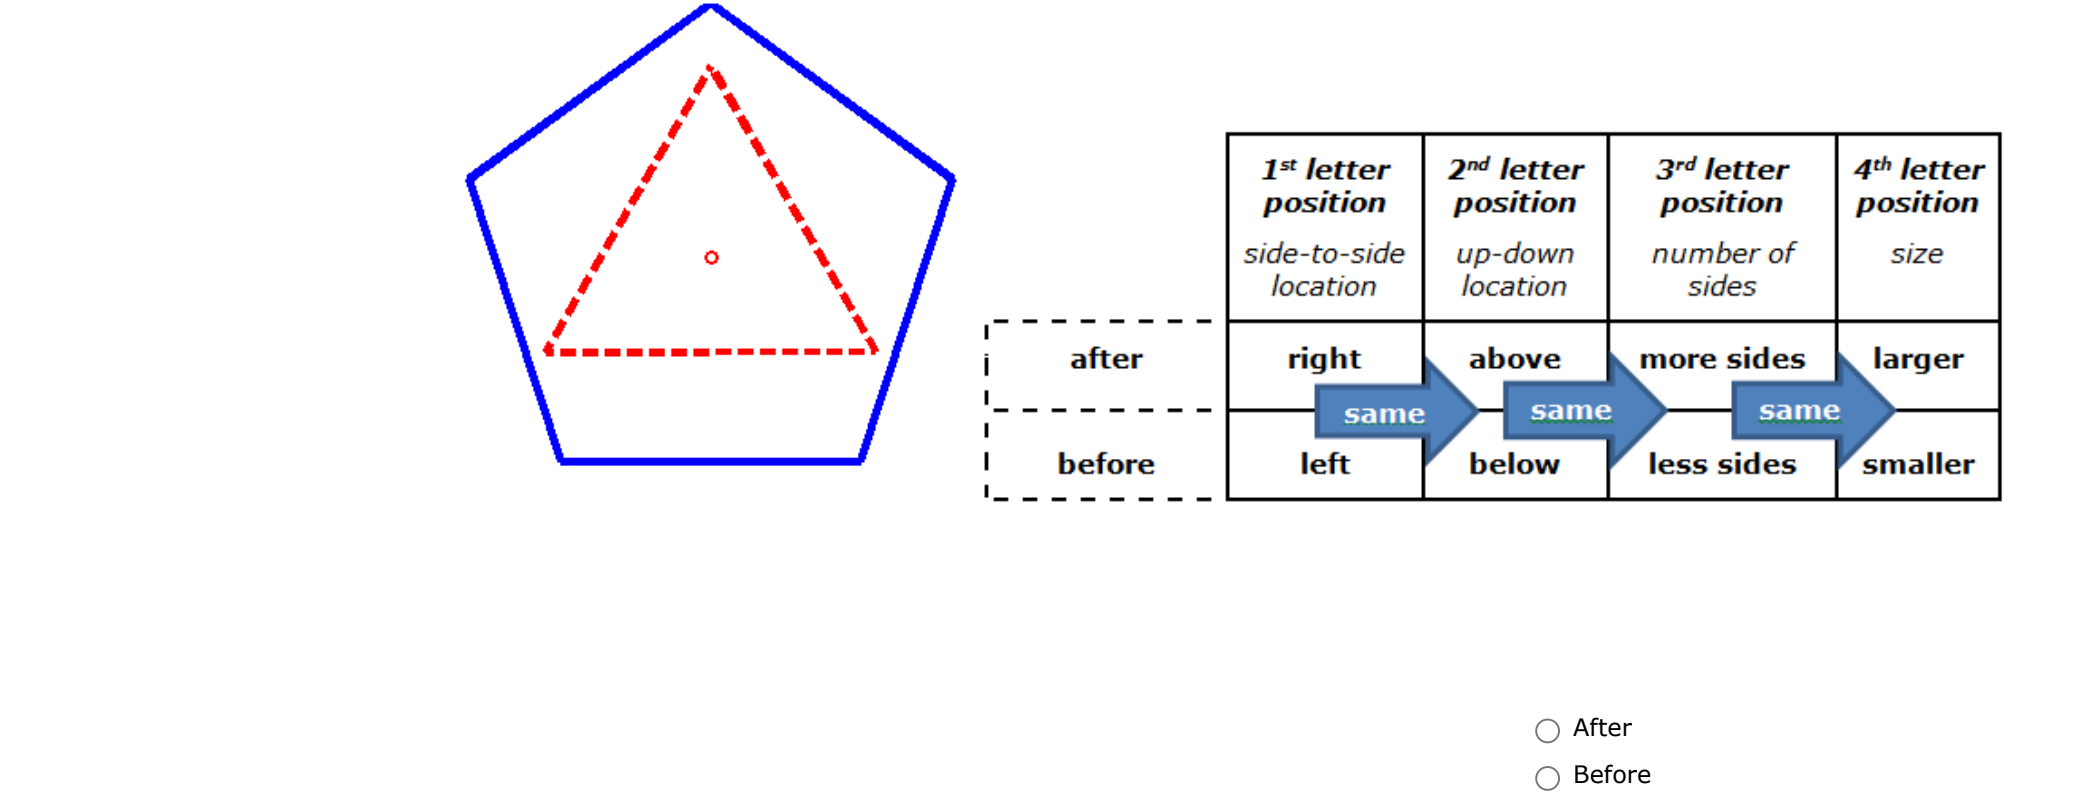

|        | 1 <sup>st</sup> letter<br>position<br>side-to-side<br>location | 2 <sup>nd</sup> letter<br>position<br>up-down<br>location | 3 <sup>rd</sup> letter<br>position<br>number of<br>sides | 4 <sup>th</sup> letter<br>position<br>size |
|--------|----------------------------------------------------------------|-----------------------------------------------------------|----------------------------------------------------------|--------------------------------------------|
| after  | right                                                          | above                                                     | more sides                                               | larger                                     |
| before | left                                                           | below                                                     | less sides                                               | smaller                                    |

☐ After  
☐ Before

5. For the image below, select whether the test shape (red dashed edges) comes after or before the reference shape (blue solid edges), as defined in the instructions above.

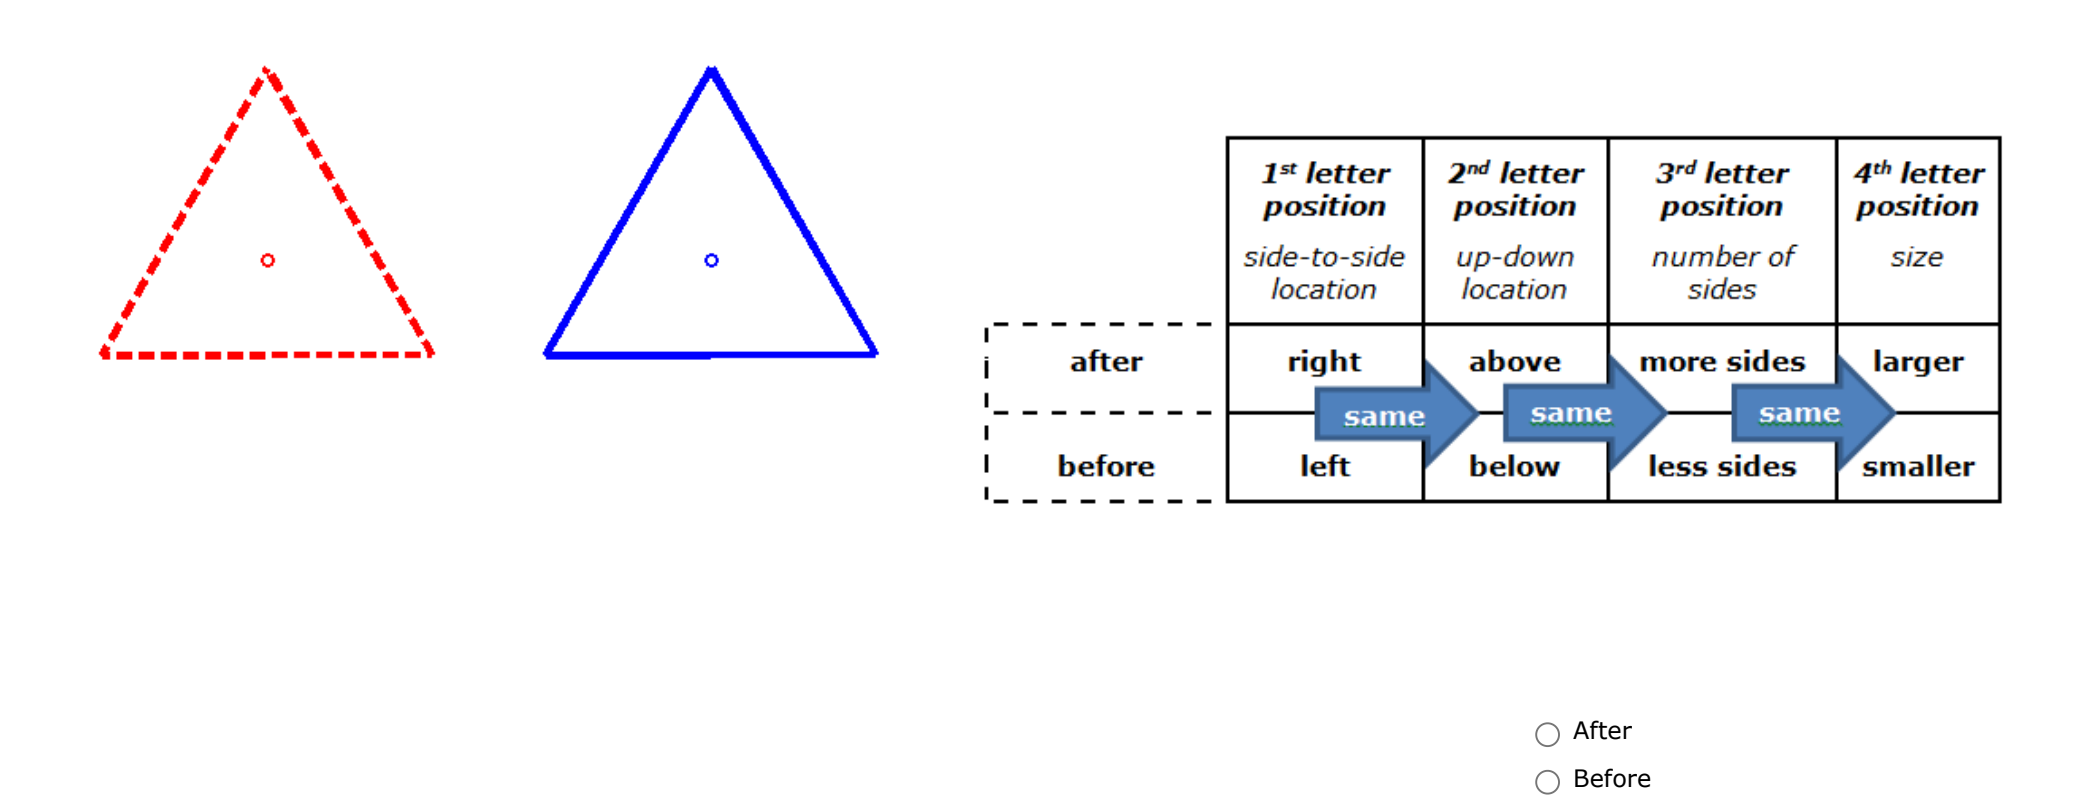

|        | 1 <sup>st</sup> letter<br>position<br>side-to-side<br>location | 2 <sup>nd</sup> letter<br>position<br>up-down<br>location | 3 <sup>rd</sup> letter<br>position<br>number of<br>sides | 4 <sup>th</sup> letter<br>position<br>size |
|--------|----------------------------------------------------------------|-----------------------------------------------------------|----------------------------------------------------------|--------------------------------------------|
| after  | right                                                          | above                                                     | more sides                                               | larger                                     |
| before | left                                                           | below                                                     | less sides                                               | smaller                                    |

☐ After  
☐ Before

6. For the image below, select whether the test shape (red dashed edges) comes after or before the reference shape (blue solid edges), as defined in the instructions above.

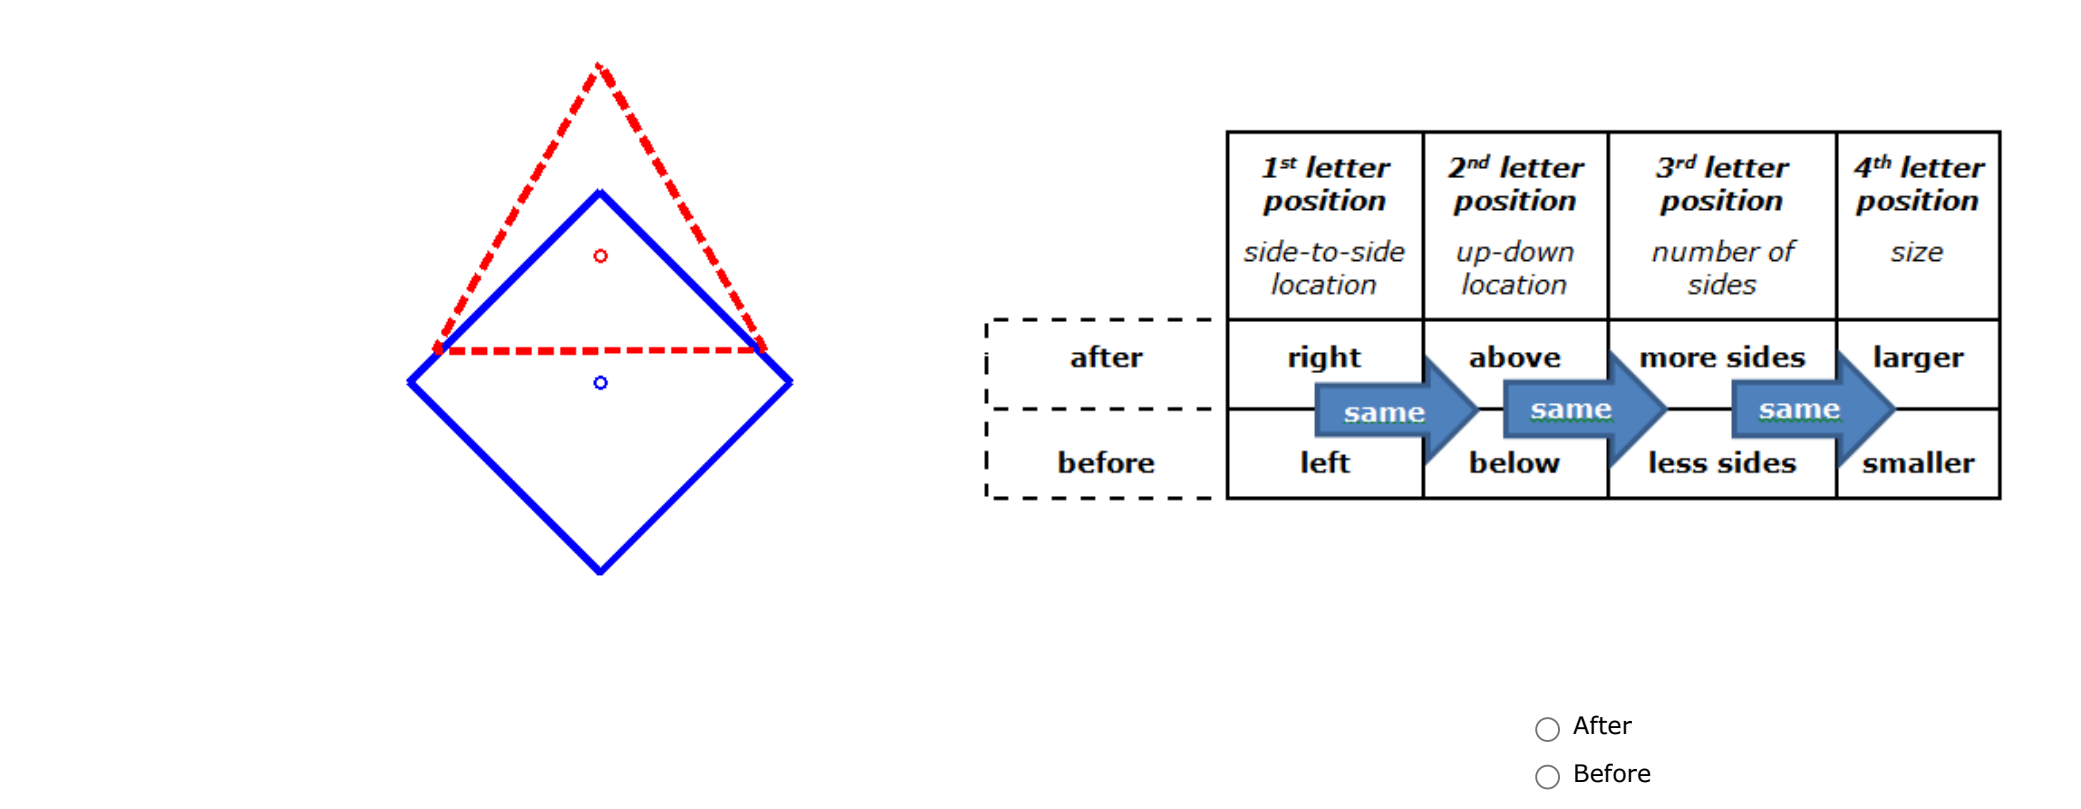

|        | 1 <sup>st</sup> letter<br>position<br>side-to-side<br>location | 2 <sup>nd</sup> letter<br>position<br>up-down<br>location | 3 <sup>rd</sup> letter<br>position<br>number of<br>sides | 4 <sup>th</sup> letter<br>position<br>size |
|--------|----------------------------------------------------------------|-----------------------------------------------------------|----------------------------------------------------------|--------------------------------------------|
| after  | right                                                          | above                                                     | more sides                                               | larger                                     |
| before | left                                                           | below                                                     | less sides                                               | smaller                                    |

☐ After  
☐ Before

7. For the image below, select whether the test shape (red dashed edges) comes after or before the reference shape (blue solid edges), as defined in the instructions above.

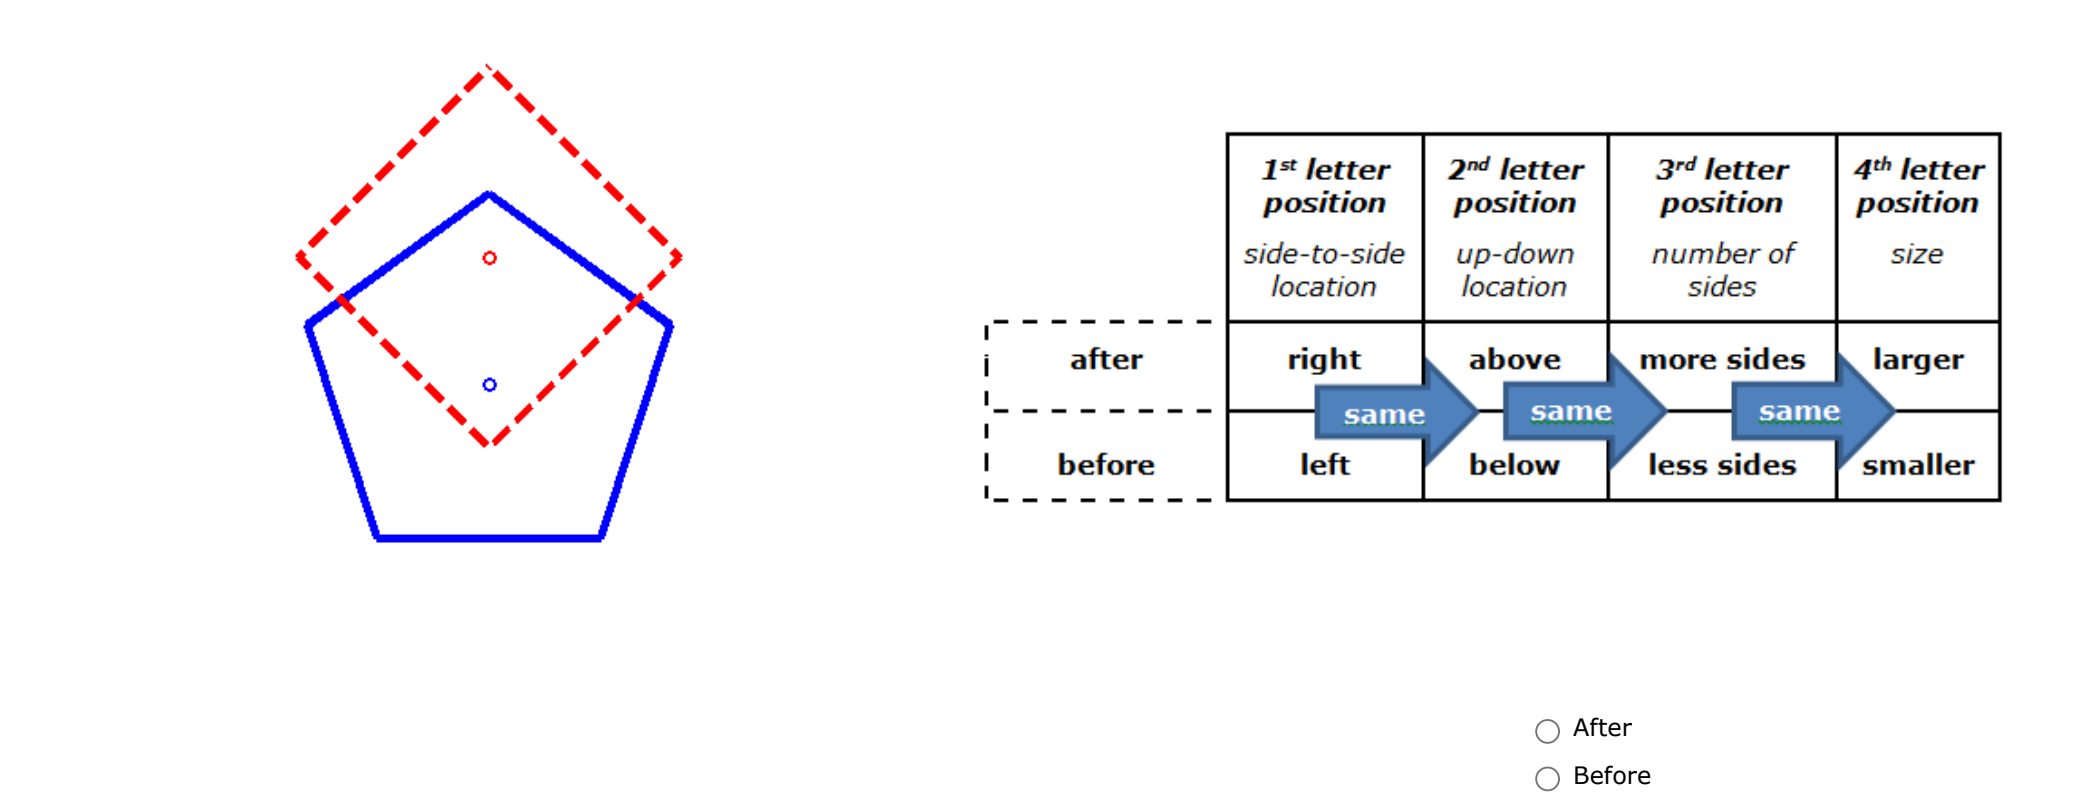

|        | 1 <sup>st</sup> letter<br>position<br>side-to-side<br>location | 2 <sup>nd</sup> letter<br>position<br>up-down<br>location | 3 <sup>rd</sup> letter<br>position<br>number of<br>sides | 4 <sup>th</sup> letter<br>position<br>size |
|--------|----------------------------------------------------------------|-----------------------------------------------------------|----------------------------------------------------------|--------------------------------------------|
| after  | right                                                          | above                                                     | more sides                                               | larger                                     |
| before | left                                                           | below                                                     | less sides                                               | smaller                                    |

☐ After  
☐ Before

8. For the image below, select whether the test shape (red dashed edges) comes after or before the reference shape (blue solid edges), as defined in the instructions above.

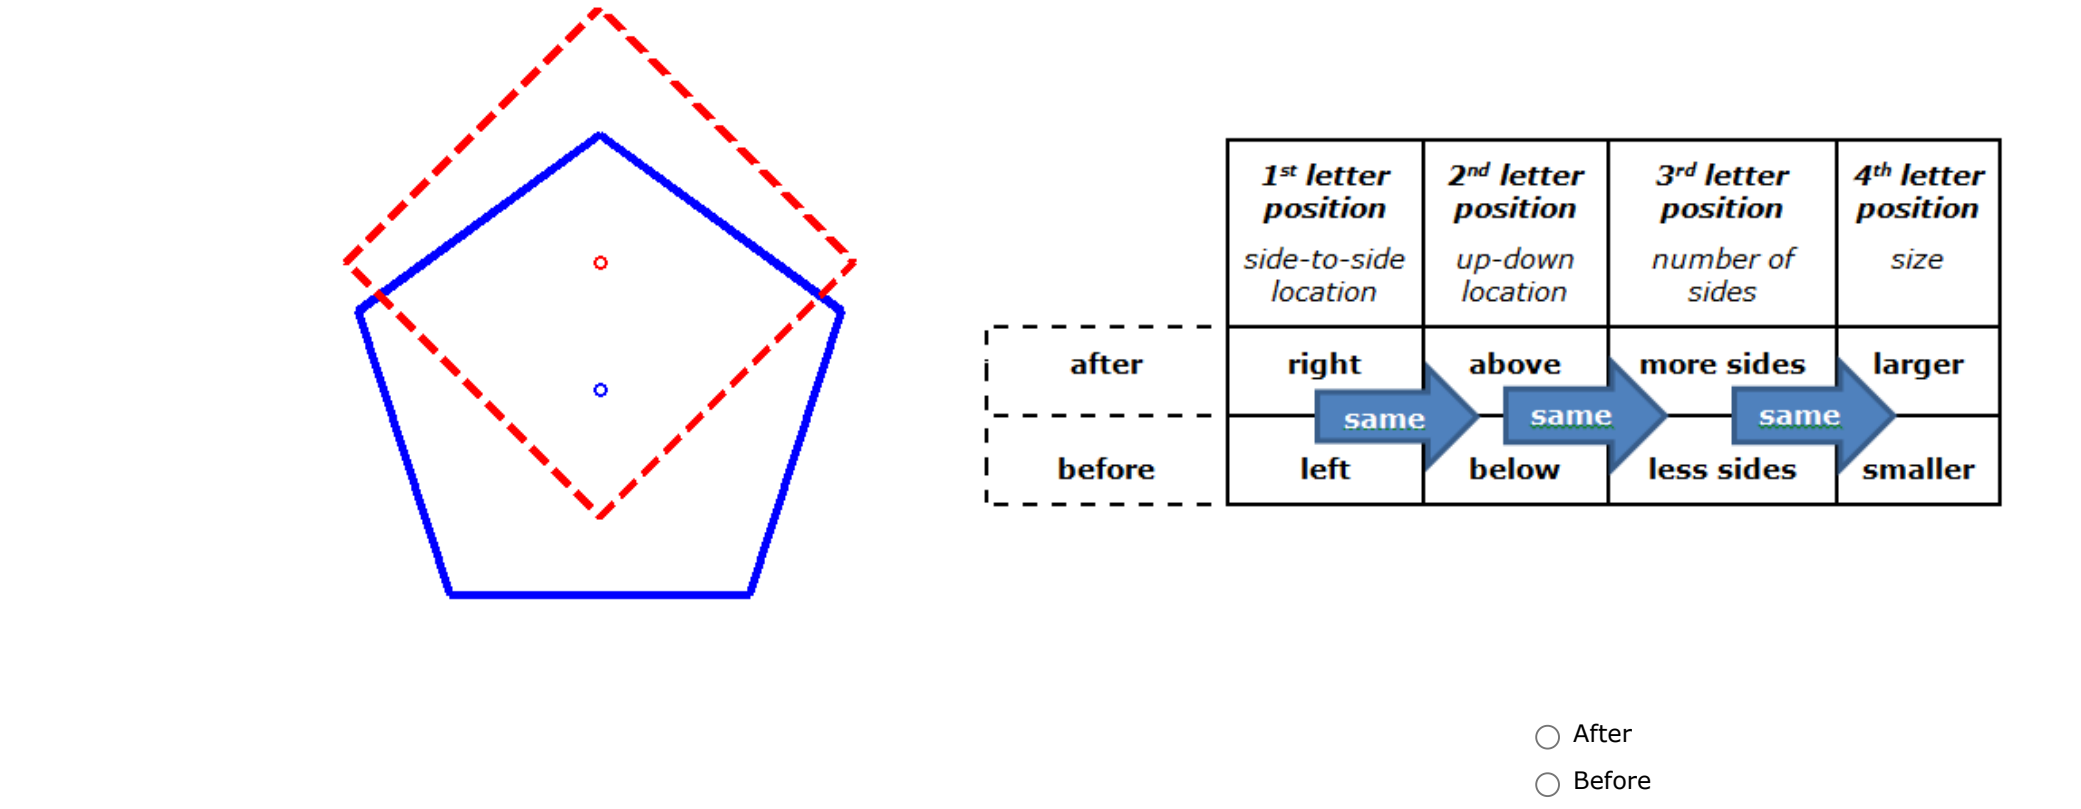

|        | 1 <sup>st</sup> letter<br>position<br>side-to-side<br>location | 2 <sup>nd</sup> letter<br>position<br>up-down<br>location | 3 <sup>rd</sup> letter<br>position<br>number of<br>sides | 4 <sup>th</sup> letter<br>position<br>size |
|--------|----------------------------------------------------------------|-----------------------------------------------------------|----------------------------------------------------------|--------------------------------------------|
| after  | right                                                          | above                                                     | more sides                                               | larger                                     |
| before | left                                                           | below                                                     | less sides                                               | smaller                                    |

☐ After  
☐ Before

9. For the image below, select whether the test shape (red dashed edges) comes after or before the reference shape (blue solid edges), as defined in the instructions above.

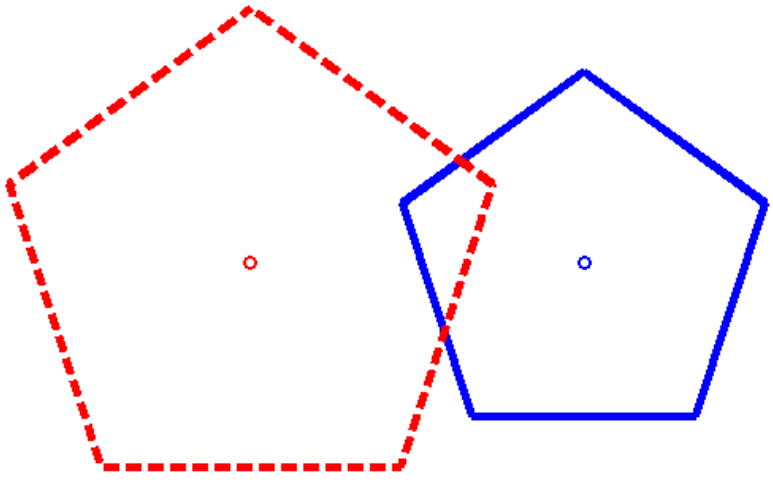

|  |        |       |       |            |         |
|--|--------|-------|-------|------------|---------|
|  | after  | right | above | more sides | larger  |
|  |        | same  | same  | same       |         |
|  | before | left  | below | less sides | smaller |

☐ After  
☐ Before

10. For the image below, select whether the test shape (red dashed edges) comes after or before the reference shape (blue solid edges), as defined in the instructions above.

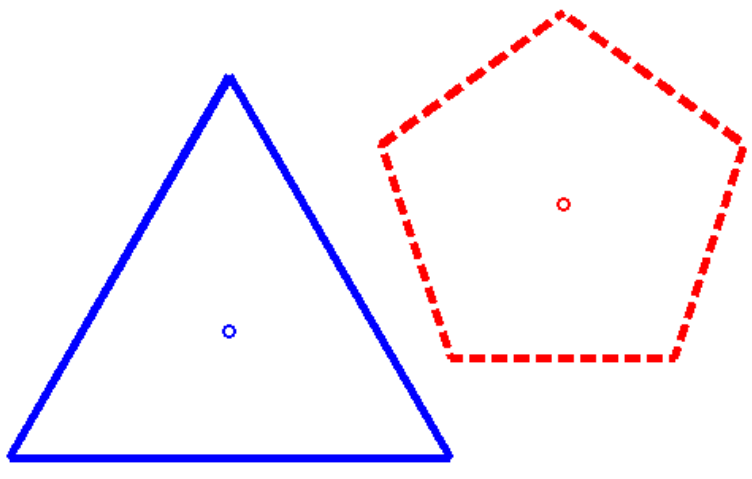

|  |        |       |       |            |         |
|--|--------|-------|-------|------------|---------|
|  | after  | right | above | more sides | larger  |
|  |        | same  | same  | same       |         |
|  | before | left  | below | less sides | smaller |

☐ After  
☐ Before

11. For the image below, select whether the test shape (red dashed edges) comes after or before the reference shape (blue solid edges), as defined in the instructions above.

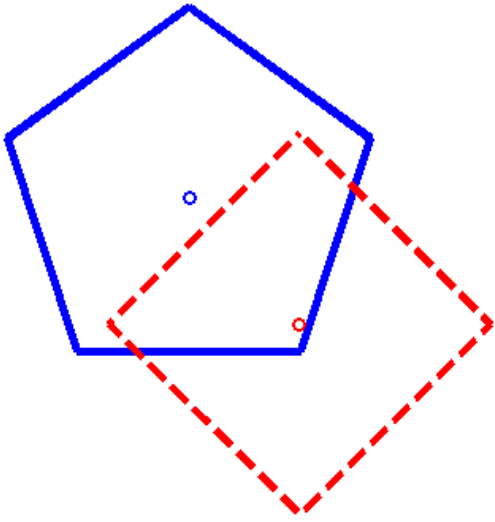

|  |        |       |       |            |         |
|--|--------|-------|-------|------------|---------|
|  | after  | right | above | more sides | larger  |
|  |        | same  | same  | same       |         |
|  | before | left  | below | less sides | smaller |

☐ After  
☐ Before

12. For the image below, select whether the test shape (red dashed edges) comes after or before the reference shape (blue solid edges), as defined in the instructions above.

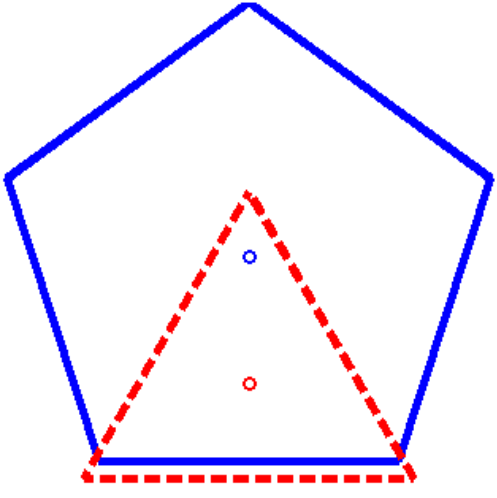

|  |        |       |       |            |         |
|--|--------|-------|-------|------------|---------|
|  | after  | right | above | more sides | larger  |
|  |        | same  | same  | same       |         |
|  | before | left  | below | less sides | smaller |

☐ After  
☐ Before

13. For the image below, select whether the test shape (red dashed edges) comes after or before the reference shape (blue solid edges), as defined in the instructions above.

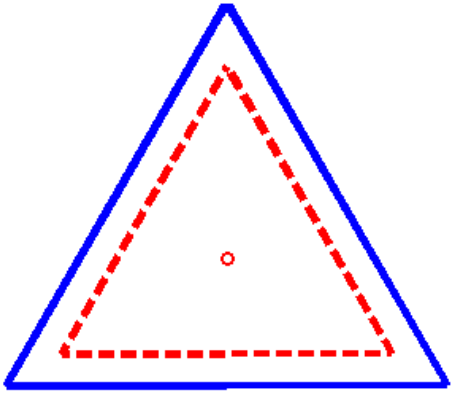

|  |        |       |       |            |         |
|--|--------|-------|-------|------------|---------|
|  | after  | right | above | more sides | larger  |
|  |        | same  | same  | same       |         |
|  | before | left  | below | less sides | smaller |

☐ After  
☐ Before

14. For the image below, select whether the test shape (red dashed edges) comes after or before the reference shape (blue solid edges), as defined in the instructions above.

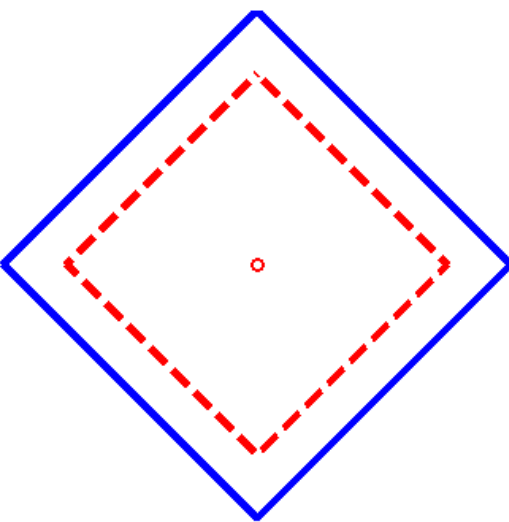

|  |        |       |       |            |         |
|--|--------|-------|-------|------------|---------|
|  | after  | right | above | more sides | larger  |
|  |        | same  | same  | same       |         |
|  | before | left  | below | less sides | smaller |

☐ After  
☐ Before

15. For the image below, select whether the test shape (red dashed edges) comes after or before the reference shape (blue solid edges), as defined in the instructions above.

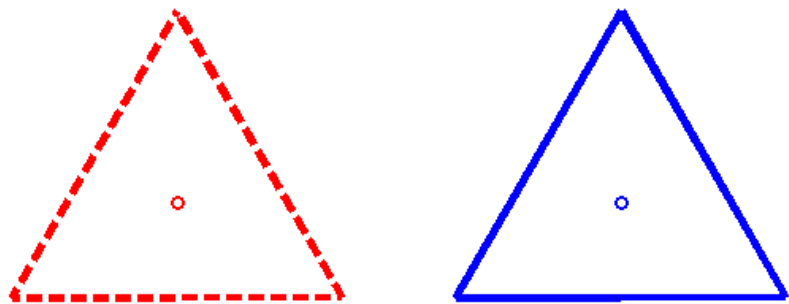

|  |        |       |       |            |         |
|--|--------|-------|-------|------------|---------|
|  | after  | right | above | more sides | larger  |
|  |        | same  | same  | same       |         |
|  | before | left  | below | less sides | smaller |

☐ After  
☐ Before

16. For the image below, select whether the test shape (red dashed edges) comes after or before the reference shape (blue solid edges), as defined in the instructions above.

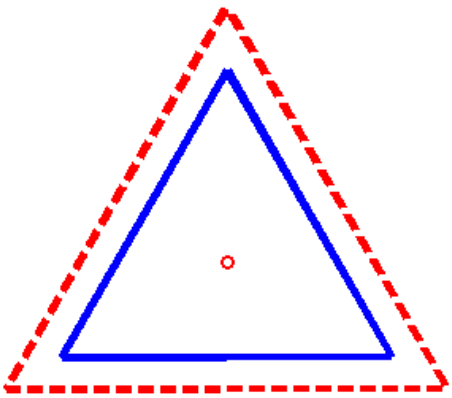

|  |        |       |       |            |         |
|--|--------|-------|-------|------------|---------|
|  | after  | right | above | more sides | larger  |
|  |        | same  | same  | same       |         |
|  | before | left  | below | less sides | smaller |

☐ After  
☐ Before

17. For the image below, select whether the test shape (red dashed edges) comes after or before the reference shape (blue solid edges), as defined in the instructions above.

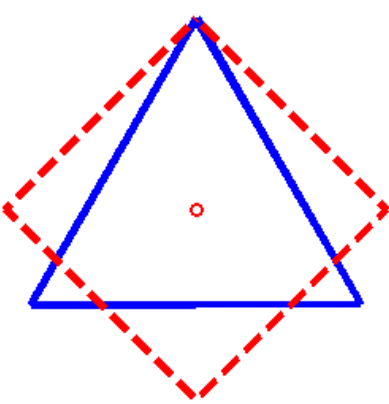

|  |        |       |       |            |         |
|--|--------|-------|-------|------------|---------|
|  | after  | right | above | more sides | larger  |
|  |        | same  | same  | same       |         |
|  | before | left  | below | less sides | smaller |

☐ After



18. For the image below, select whether the test shape (red dashed edges) comes after or before the reference shape (blue solid edges), as defined in the instructions above.

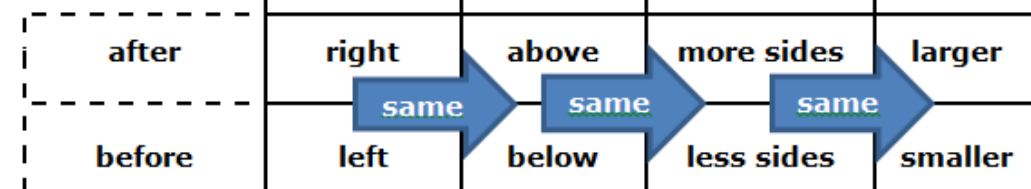

19. For the image below, select whether the test shape (red dashed edges) comes after or before the reference shape (blue solid edges), as defined in the instructions above.

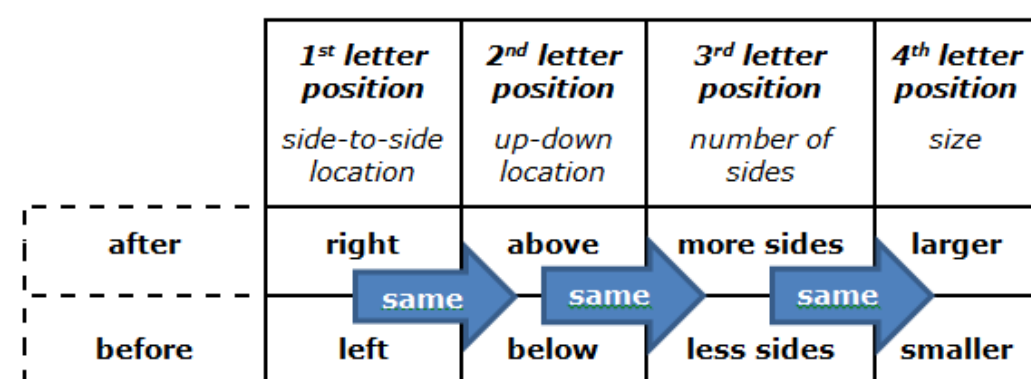

20. For the image below, select whether the test shape (red dashed edges) comes after or before the reference shape (blue solid edges), as defined in the instructions above.

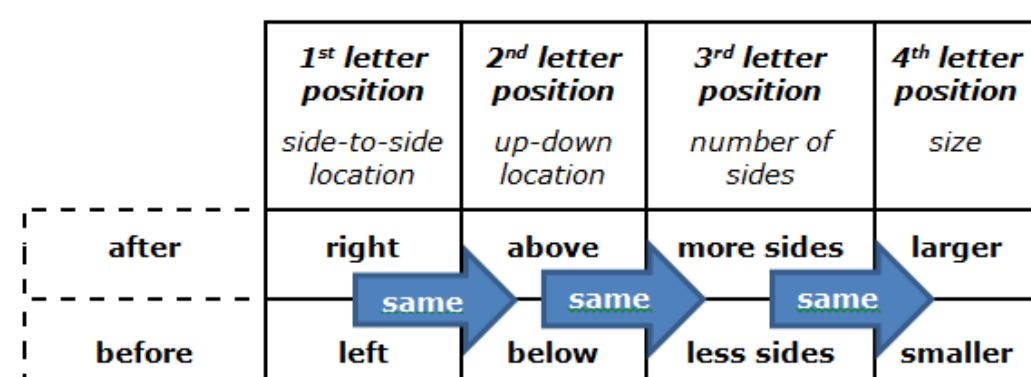

21. For the image below, select whether the test shape (red dashed edges) comes after or before the reference shape (blue solid edges), as defined in the instructions above.

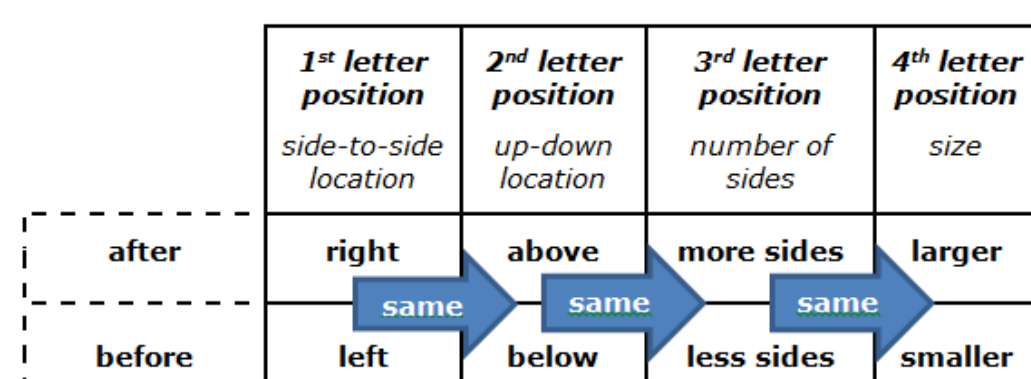

22. For the image below, select whether the test shape (red dashed edges) comes after or before the reference shape (blue solid edges), as defined in the instructions above.

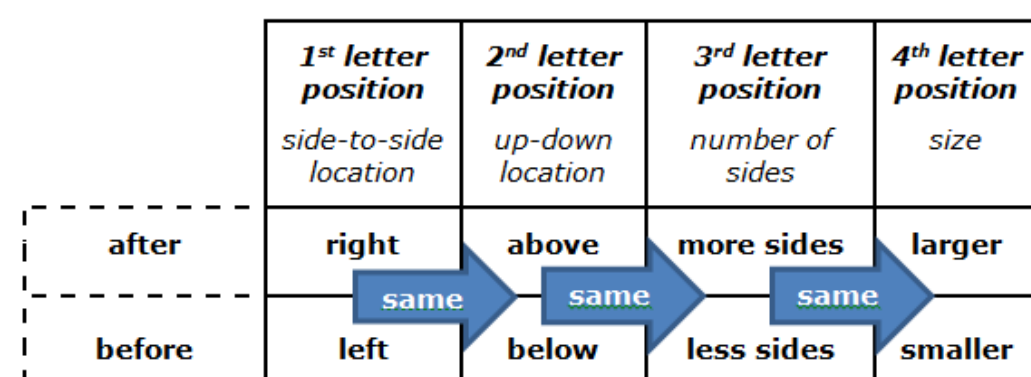

23. For the image below, select whether the test shape (red dashed edges) comes after or before the reference shape (blue solid edges), as defined in the instructions above.

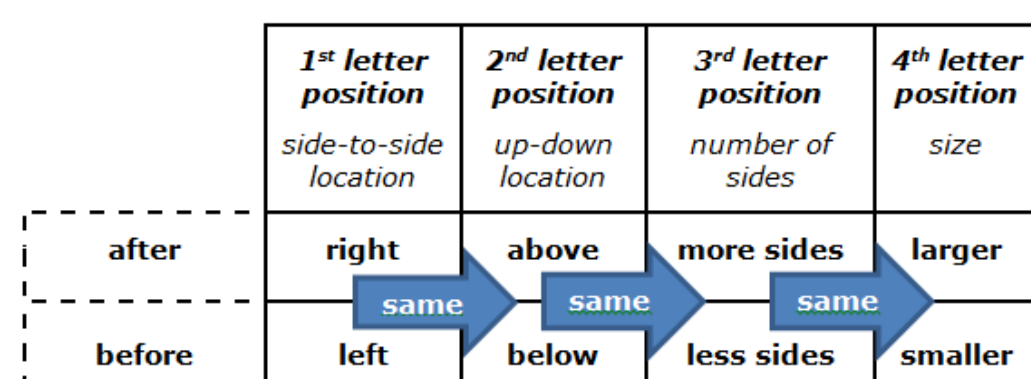

24. For the image below, select whether the test shape (red dashed edges) comes after or before the reference shape (blue solid edges), as defined in the instructions above.

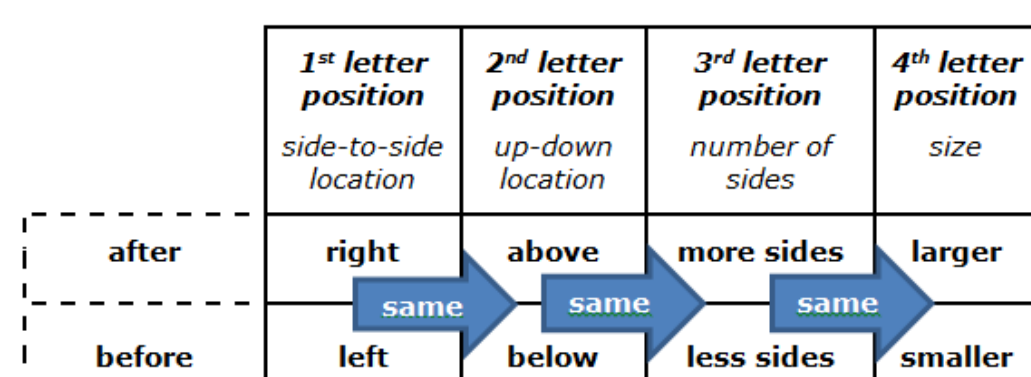

25. For the image below, select whether the test shape (red dashed edges) comes after or before the reference shape (blue solid edges), as defined in the instructions above.

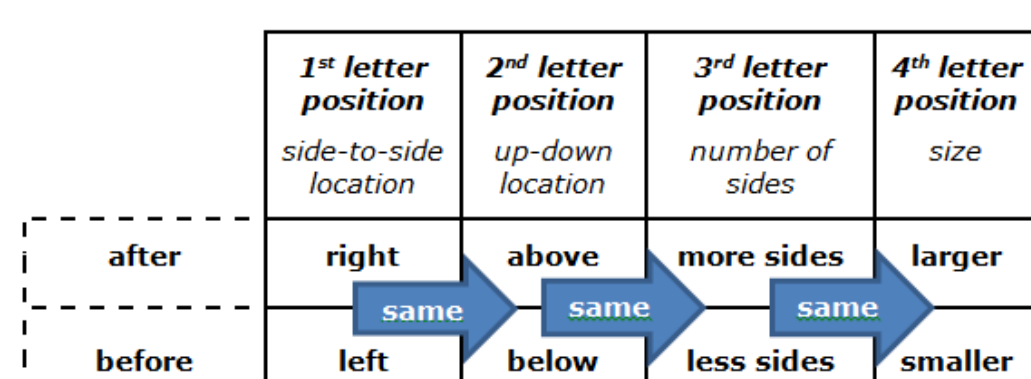

26. For the image below, select whether the test shape (red dashed edges) comes after or before the reference shape (blue solid edges), as defined in the instructions above.





☐ Before

35. For the image below, select whether the test shape (red dashed edges) comes after or before the reference shape (blue solid edges), as defined in the instructions above.

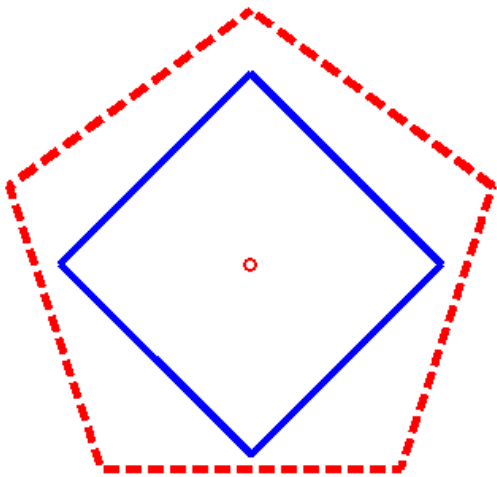

|        | 1 <sup>st</sup> letter<br>position<br>side-to-side<br>location | 2 <sup>nd</sup> letter<br>position<br>up-down<br>location | 3 <sup>rd</sup> letter<br>position<br>number of<br>sides | 4 <sup>th</sup> letter<br>position<br>size |
|--------|----------------------------------------------------------------|-----------------------------------------------------------|----------------------------------------------------------|--------------------------------------------|
| after  | right                                                          | above                                                     | more sides                                               | larger                                     |
| before | left                                                           | below                                                     | less sides                                               | smaller                                    |

☐ After  
☐ Before

36. For the image below, select whether the test shape (red dashed edges) comes after or before the reference shape (blue solid edges), as defined in the instructions above.

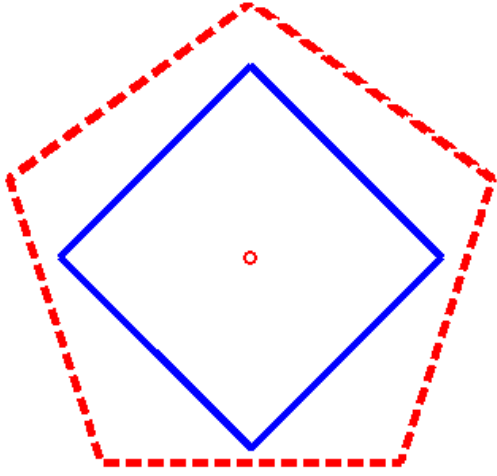

|        | 1 <sup>st</sup> letter<br>position<br>side-to-side<br>location | 2 <sup>nd</sup> letter<br>position<br>up-down<br>location | 3 <sup>rd</sup> letter<br>position<br>number of<br>sides | 4 <sup>th</sup> letter<br>position<br>size |
|--------|----------------------------------------------------------------|-----------------------------------------------------------|----------------------------------------------------------|--------------------------------------------|
| after  | right                                                          | above                                                     | more sides                                               | larger                                     |
| before | left                                                           | below                                                     | less sides                                               | smaller                                    |

☐ After  
☐ Before

37. For the image below, select whether the test shape (red dashed edges) comes after or before the reference shape (blue solid edges), as defined in the instructions above.

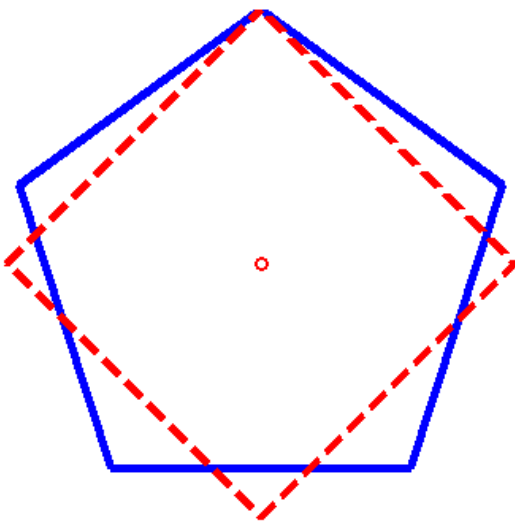

|        | 1 <sup>st</sup> letter<br>position<br>side-to-side<br>location | 2 <sup>nd</sup> letter<br>position<br>up-down<br>location | 3 <sup>rd</sup> letter<br>position<br>number of<br>sides | 4 <sup>th</sup> letter<br>position<br>size |
|--------|----------------------------------------------------------------|-----------------------------------------------------------|----------------------------------------------------------|--------------------------------------------|
| after  | right                                                          | above                                                     | more sides                                               | larger                                     |
| before | left                                                           | below                                                     | less sides                                               | smaller                                    |

☐ After  
☐ Before

38. For the image below, select whether the test shape (red dashed edges) comes after or before the reference shape (blue solid edges), as defined in the instructions above.

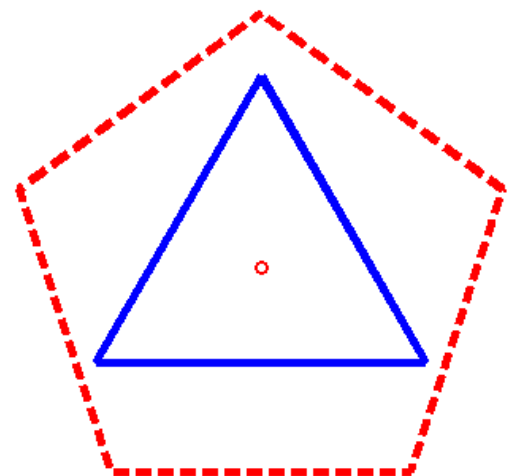

|        | 1 <sup>st</sup> letter<br>position<br>side-to-side<br>location | 2 <sup>nd</sup> letter<br>position<br>up-down<br>location | 3 <sup>rd</sup> letter<br>position<br>number of<br>sides | 4 <sup>th</sup> letter<br>position<br>size |
|--------|----------------------------------------------------------------|-----------------------------------------------------------|----------------------------------------------------------|--------------------------------------------|
| after  | right                                                          | above                                                     | more sides                                               | larger                                     |
| before | left                                                           | below                                                     | less sides                                               | smaller                                    |

☐ After  
☐ Before

39. For the image below, select whether the test shape (red dashed edges) comes after or before the reference shape (blue solid edges), as defined in the instructions above.

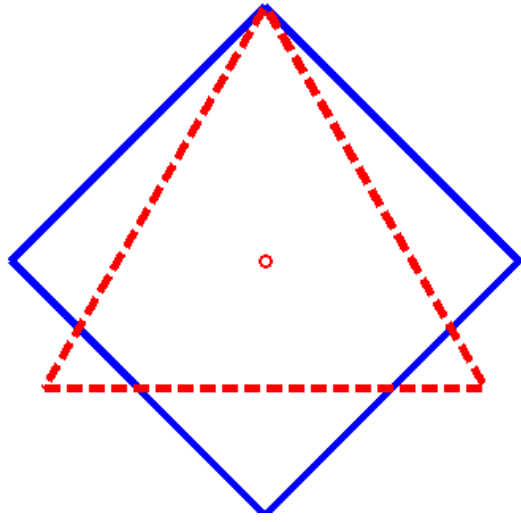

|        | 1 <sup>st</sup> letter<br>position<br>side-to-side<br>location | 2 <sup>nd</sup> letter<br>position<br>up-down<br>location | 3 <sup>rd</sup> letter<br>position<br>number of<br>sides | 4 <sup>th</sup> letter<br>position<br>size |
|--------|----------------------------------------------------------------|-----------------------------------------------------------|----------------------------------------------------------|--------------------------------------------|
| after  | right                                                          | above                                                     | more sides                                               | larger                                     |
| before | left                                                           | below                                                     | less sides                                               | smaller                                    |

☐ After  
☐ Before

40. For the image below, select whether the test shape (red dashed edges) comes after or before the reference shape (blue solid edges), as defined in the instructions above.

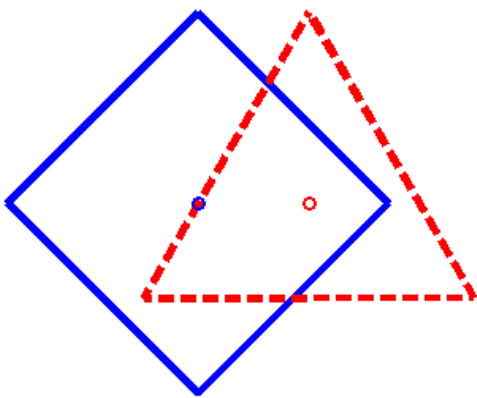

|        | 1 <sup>st</sup> letter<br>position<br>side-to-side<br>location | 2 <sup>nd</sup> letter<br>position<br>up-down<br>location | 3 <sup>rd</sup> letter<br>position<br>number of<br>sides | 4 <sup>th</sup> letter<br>position<br>size |
|--------|----------------------------------------------------------------|-----------------------------------------------------------|----------------------------------------------------------|--------------------------------------------|
| after  | right                                                          | above                                                     | more sides                                               | larger                                     |
| before | left                                                           | below                                                     | less sides                                               | smaller                                    |

☐ After  
☐ Before

41. For the image below, select whether the test shape (red dashed edges) comes after or before the reference shape (blue solid edges), as defined in the instructions above.

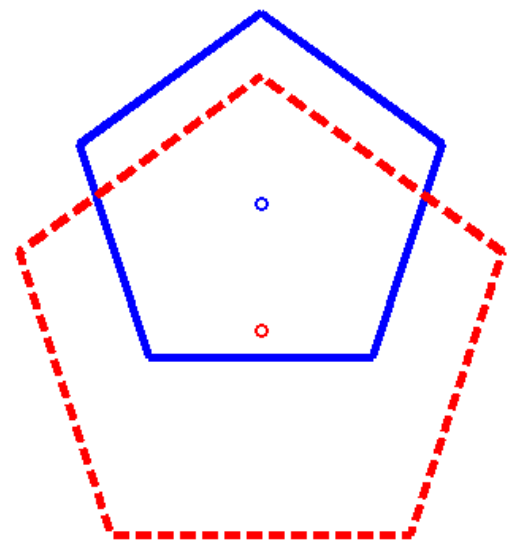

|        | 1 <sup>st</sup> letter<br>position<br>side-to-side<br>location | 2 <sup>nd</sup> letter<br>position<br>up-down<br>location | 3 <sup>rd</sup> letter<br>position<br>number of<br>sides | 4 <sup>th</sup> letter<br>position<br>size |
|--------|----------------------------------------------------------------|-----------------------------------------------------------|----------------------------------------------------------|--------------------------------------------|
| after  | right                                                          | above                                                     | more sides                                               | larger                                     |
| before | left                                                           | below                                                     | less sides                                               | smaller                                    |

☐ After  
☐ Before

42. For the image below, select whether the test shape (red dashed edges) comes after or before the reference shape (blue solid edges), as defined in the instructions above.

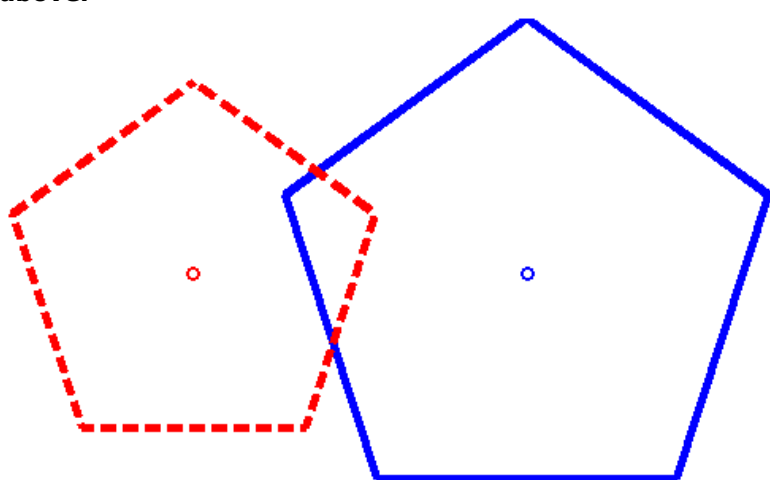

|        | 1 <sup>st</sup> letter<br>position<br>side-to-side<br>location | 2 <sup>nd</sup> letter<br>position<br>up-down<br>location | 3 <sup>rd</sup> letter<br>position<br>number of<br>sides | 4 <sup>th</sup> letter<br>position<br>size |
|--------|----------------------------------------------------------------|-----------------------------------------------------------|----------------------------------------------------------|--------------------------------------------|
| after  | right                                                          | above                                                     | more sides                                               | larger                                     |
| before | left                                                           | below                                                     | less sides                                               | smaller                                    |

☐ After  
☐ Before

43. For the image below, select whether the test shape (red dashed edges) comes after or before the reference shape (blue solid edges), as defined in the instructions above.





52. For the image below, select whether the test shape (red dashed edges) comes after or before the reference shape (blue solid edges), as defined in the instructions above.

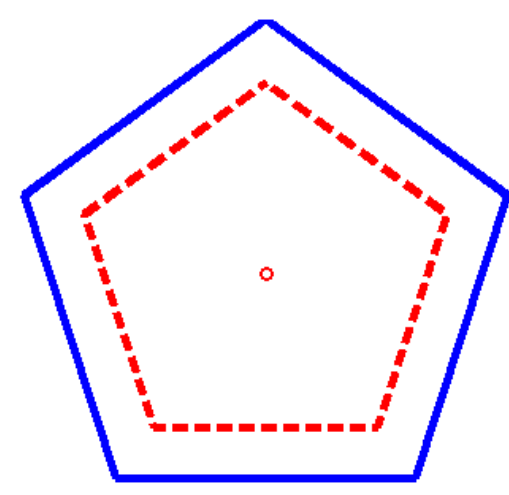

|        | 1 <sup>st</sup> letter position<br><i>side-to-side</i><br>location | 2 <sup>nd</sup> letter position<br><i>up-down</i><br>location | 3 <sup>rd</sup> letter position<br><i>number of</i><br>sides | 4 <sup>th</sup> letter position<br><i>size</i> |
|--------|--------------------------------------------------------------------|---------------------------------------------------------------|--------------------------------------------------------------|------------------------------------------------|
| after  | right                                                              | above                                                         | more sides                                                   | larger                                         |
| before | left                                                               | below                                                         | less sides                                                   | smaller                                        |

☐ Before

53. For the image below, select whether the test shape (red dashed edges) comes after or before the reference shape (blue solid edges), as defined in the instructions above.

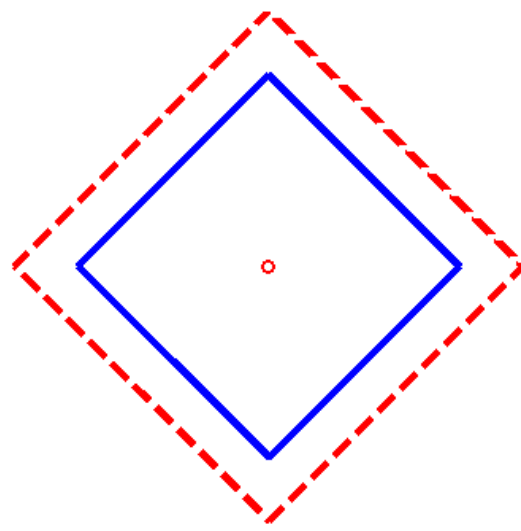

|        | 1 <sup>st</sup> letter position<br><i>side-to-side location</i> | 2 <sup>nd</sup> letter position<br><i>up-down location</i> | 3 <sup>rd</sup> letter position<br><i>number of sides</i> | 4 <sup>th</sup> letter position<br><i>size</i> |
|--------|-----------------------------------------------------------------|------------------------------------------------------------|-----------------------------------------------------------|------------------------------------------------|
| after  | right                                                           | above                                                      | more sides                                                | larger                                         |
| before | left                                                            | below                                                      | less sides                                                | smaller                                        |

☐ Before

54. For the image below, select whether the test shape (red dashed edges) comes after or before the reference shape (blue solid edges), as defined in the instructions above.

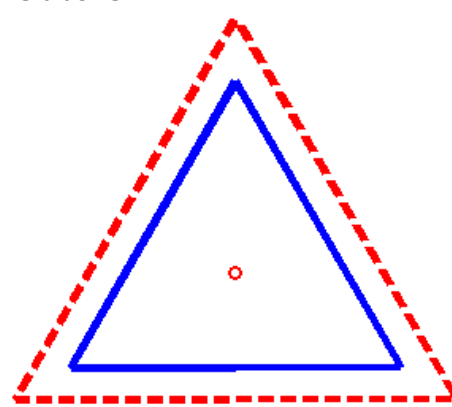

|        | 1 <sup>st</sup> letter position<br><i>side-to-side location</i> | 2 <sup>nd</sup> letter position<br><i>up-down location</i> | 3 <sup>rd</sup> letter position<br><i>number of sides</i> | 4 <sup>th</sup> letter position<br><i>size</i> |
|--------|-----------------------------------------------------------------|------------------------------------------------------------|-----------------------------------------------------------|------------------------------------------------|
| after  | right                                                           | above                                                      | more sides                                                | larger                                         |
| before | left                                                            | below                                                      | less sides                                                | smaller                                        |

☐ Before

55. For the image below, select whether the test shape (red dashed edges) comes after or before the reference shape (blue solid edges), as defined in the instructions above.

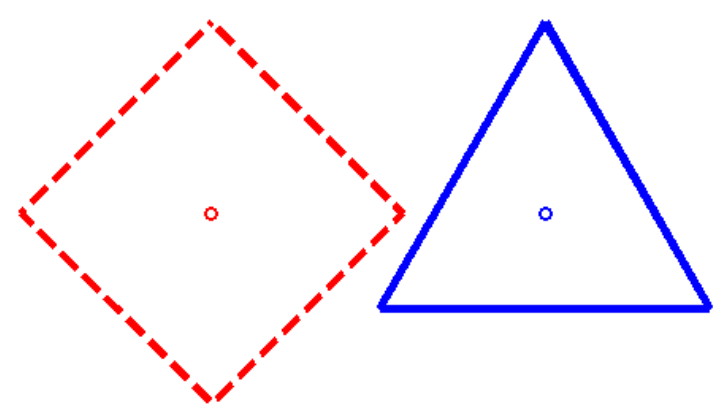

|        | 1 <sup>st</sup> letter position<br><i>side-to-side</i><br>location | 2 <sup>nd</sup> letter position<br><i>up-down</i><br>location | 3 <sup>rd</sup> letter position<br><i>number of</i><br>sides | 4 <sup>th</sup> letter position<br><i>size</i> |
|--------|--------------------------------------------------------------------|---------------------------------------------------------------|--------------------------------------------------------------|------------------------------------------------|
| after  | right                                                              | above                                                         | more sides                                                   | larger                                         |
| before | left                                                               | below                                                         | less sides                                                   | smaller                                        |

☐ Before

56. For the image below, select whether the test shape (red dashed edges) comes after or before the reference shape (blue solid edges), as defined in the instructions above.

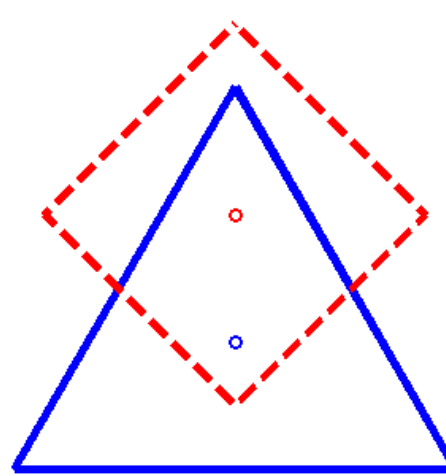

|        | 1 <sup>st</sup> letter position<br><i>side-to-side location</i> | 2 <sup>nd</sup> letter position<br><i>up-down location</i> | 3 <sup>rd</sup> letter position<br><i>number of sides</i> | 4 <sup>th</sup> letter position<br><i>size</i> |
|--------|-----------------------------------------------------------------|------------------------------------------------------------|-----------------------------------------------------------|------------------------------------------------|
| after  | right                                                           | above                                                      | more sides                                                | larger                                         |
| before | left                                                            | below                                                      | less sides                                                | smaller                                        |

☐ After

☐ Before

57. For the image below, select whether the test shape (red dashed edges) comes after or before the reference shape (blue solid edges), as defined in the instructions above.

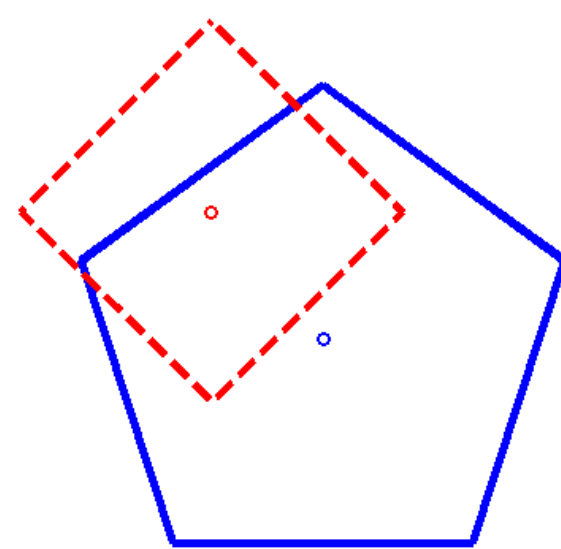

|        | 1 <sup>st</sup> letter position<br><i>side-to-side</i><br>location | 2 <sup>nd</sup> letter position<br><i>up-down</i><br>location | 3 <sup>rd</sup> letter position<br>number of<br>sides | 4 <sup>th</sup> letter position<br>size |
|--------|--------------------------------------------------------------------|---------------------------------------------------------------|-------------------------------------------------------|-----------------------------------------|
| after  | right                                                              | above                                                         | more sides                                            | larger                                  |
| before | left                                                               | below                                                         | less sides                                            | smaller                                 |

☐ Before

58. For the image below, select whether the test shape (red dashed edges) comes after or before the reference shape (blue solid edges), as defined in the instructions above.

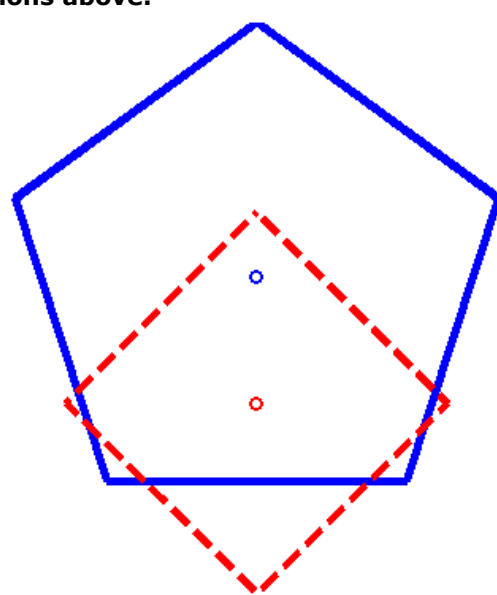

|        | 1 <sup>st</sup> letter position<br>side-to-side location | 2 <sup>nd</sup> letter position<br>up-down location | 3 <sup>rd</sup> letter position<br>number of sides | 4 <sup>th</sup> letter position<br>size |
|--------|----------------------------------------------------------|-----------------------------------------------------|----------------------------------------------------|-----------------------------------------|
| after  | right                                                    | above                                               | more sides                                         | larger                                  |
| before | left                                                     | below                                               | less sides                                         | smaller                                 |

☐ Before

59. For the image below, select whether the test shape (red dashed edges) comes after or before the reference shape (blue solid edges), as defined in the instructions above.

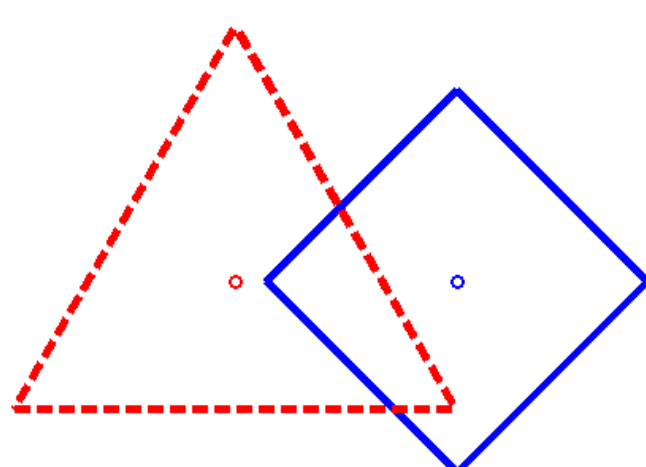

|        | 1 <sup>st</sup> letter position<br><i>side-to-side location</i> | 2 <sup>nd</sup> letter position<br><i>up-down location</i> | 3 <sup>rd</sup> letter position<br><i>number of sides</i> | 4 <sup>th</sup> letter position<br><i>size</i> |
|--------|-----------------------------------------------------------------|------------------------------------------------------------|-----------------------------------------------------------|------------------------------------------------|
| after  | right                                                           | above                                                      | more sides                                                | larger                                         |
| before | left                                                            | below                                                      | less sides                                                | smaller                                        |

☐ After

☐ Before

60. For the image below, select whether the test shape (red dashed edges) comes after or before the reference shape (blue solid edges), as defined in the instructions above.



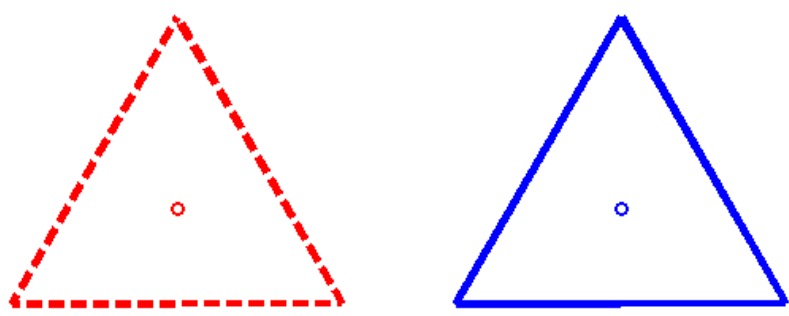

|  |        |       |       |            |         |
|--|--------|-------|-------|------------|---------|
|  | after  | right | above | more sides | larger  |
|  |        | same  | same  | same       |         |
|  | before | left  | below | less sides | smaller |

- ☐ After  
☐ Before

61. For the image below, select whether the test shape (red dashed edges) comes after or before the reference shape (blue solid edges), as defined in the instructions above.

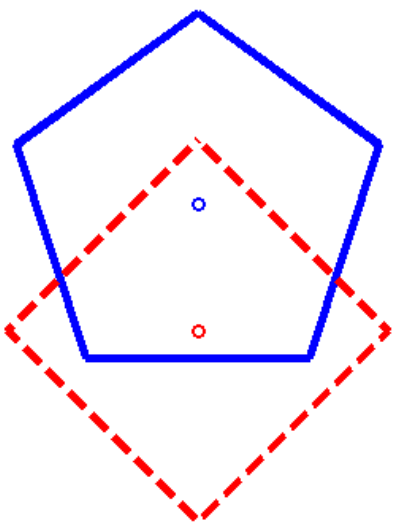

|  |        |       |       |            |         |
|--|--------|-------|-------|------------|---------|
|  | after  | right | above | more sides | larger  |
|  |        | same  | same  | same       |         |
|  | before | left  | below | less sides | smaller |

- ☐ After  
☐ Before

62. For the image below, select whether the test shape (red dashed edges) comes after or before the reference shape (blue solid edges), as defined in the instructions above.

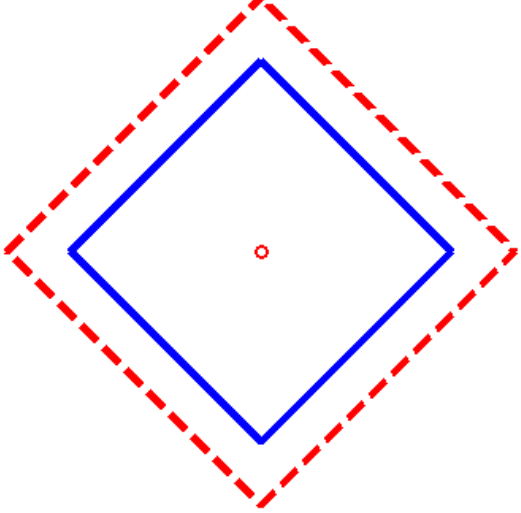

|  |        |       |       |            |         |
|--|--------|-------|-------|------------|---------|
|  | after  | right | above | more sides | larger  |
|  |        | same  | same  | same       |         |
|  | before | left  | below | less sides | smaller |

- ☐ After  
☐ Before

63. For the image below, select whether the test shape (red dashed edges) comes after or before the reference shape (blue solid edges), as defined in the instructions above.

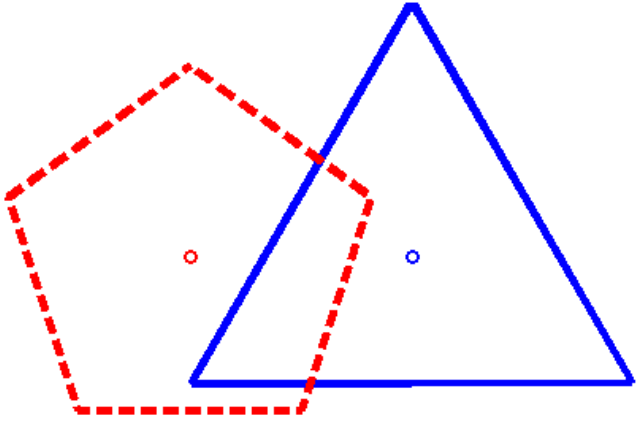

|  |        |       |       |            |         |
|--|--------|-------|-------|------------|---------|
|  | after  | right | above | more sides | larger  |
|  |        | same  | same  | same       |         |
|  | before | left  | below | less sides | smaller |

- ☐ After  
☐ Before

64. For the image below, select whether the test shape (red dashed edges) comes after or before the reference shape (blue solid edges), as defined in the instructions above.

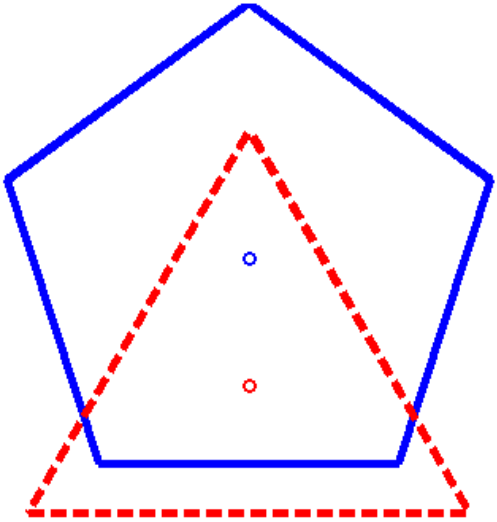

|  |        |       |       |            |         |
|--|--------|-------|-------|------------|---------|
|  | after  | right | above | more sides | larger  |
|  |        | same  | same  | same       |         |
|  | before | left  | below | less sides | smaller |

- ☐ After  
☐ Before

65. For the image below, select whether the test shape (red dashed edges) comes after or before the reference shape (blue solid edges), as defined in the instructions above.

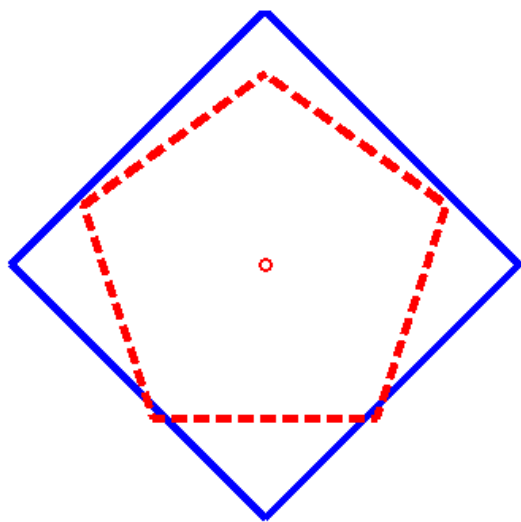

|  |        |       |       |            |         |
|--|--------|-------|-------|------------|---------|
|  | after  | right | above | more sides | larger  |
|  |        | same  | same  | same       |         |
|  | before | left  | below | less sides | smaller |

- ☐ After  
☐ Before

66. For the image below, select whether the test shape (red dashed edges) comes after or before the reference shape (blue solid edges), as defined in the instructions above.

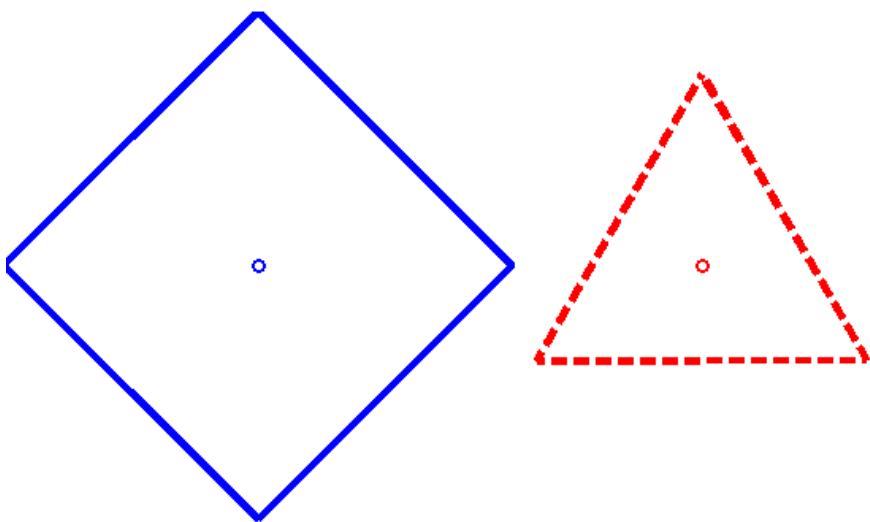

|  |        |       |       |            |         |
|--|--------|-------|-------|------------|---------|
|  | after  | right | above | more sides | larger  |
|  |        | same  | same  | same       |         |
|  | before | left  | below | less sides | smaller |

- ☐ After  
☐ Before

67. For the image below, select whether the test shape (red dashed edges) comes after or before the reference shape (blue solid edges), as defined in the instructions above.

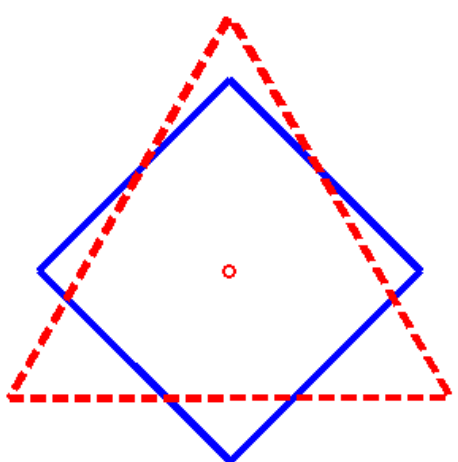

|  |        |       |       |            |         |
|--|--------|-------|-------|------------|---------|
|  | after  | right | above | more sides | larger  |
|  |        | same  | same  | same       |         |
|  | before | left  | below | less sides | smaller |

- ☐ After  
☐ Before

68. For the image below, select whether the test shape (red dashed edges) comes after or before the reference shape (blue solid edges), as defined in the instructions above.

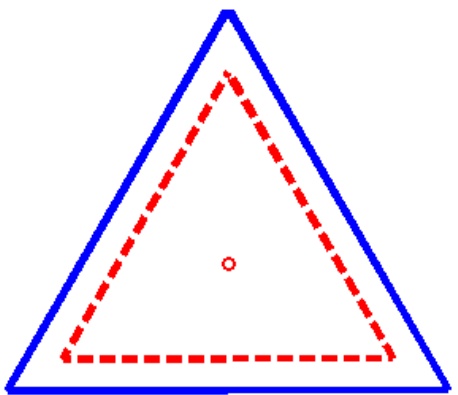

|  |        |       |       |            |         |
|--|--------|-------|-------|------------|---------|
|  | after  | right | above | more sides | larger  |
|  |        | same  | same  | same       |         |
|  | before | left  | below | less sides | smaller |

- ☐ After

69. For the image below, select whether the test shape (red dashed edges) comes after or before the reference shape (blue solid edges), as defined in the instructions above.

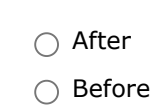

70. For the image below, select whether the test shape (red dashed edges) comes after or before the reference shape (blue solid edges), as defined in the instructions above.

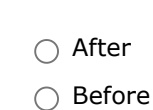

71. For the image below, select whether the test shape (red dashed edges) comes after or before the reference shape (blue solid edges), as defined in the instructions above.

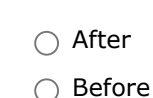

72. For the image below, select whether the test shape (red dashed edges) comes after or before the reference shape (blue solid edges), as defined in the instructions above.

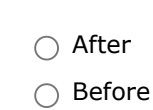

73. For the image below, select whether the test shape (red dashed edges) comes after or before the reference shape (blue solid edges), as defined in the instructions above.

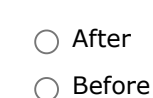

74. For the image below, select whether the test shape (red dashed edges) comes after or before the reference shape (blue solid edges), as defined in the instructions above.

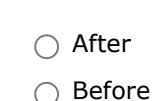

75. For the image below, select whether the test shape (red dashed edges) comes after or before the reference shape (blue solid edges), as defined in the instructions above.

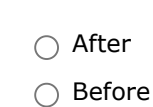

76. For the image below, select whether the test shape (red dashed edges) comes after or before the reference shape (blue solid edges), as defined in the instructions above.

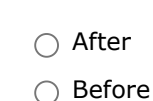

77. For the image below, select whether the test shape (red dashed edges) comes after or before the reference shape (blue solid edges), as defined in the instructions above.



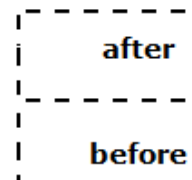

☐ After

☐ Before

☐ After

☐ Before

A diagram showing a blue triangle with a dashed red pentagon inside it. The pentagon is oriented with one vertex pointing upwards. There are two small circles inside the triangle: a red one near the top vertex and a blue one near the bottom vertex.

☐ After

☐ Before

☐ After

☐ Before

A diagram of a regular pentagon. It features a dashed red outer boundary and a solid blue inner boundary. A small red dot is located at the center of the pentagon.

☐ After

☐ Before

A diagram showing a diamond-shaped region. The outer boundary is a solid blue line. Inside it is a dashed red line forming a smaller diamond. At the center of the dashed red diamond is a small red dot.

☐ After

☐ Before

☐ After

☐ Before

A diagram showing a blue triangle with a red dashed pentagon around it. A small red circle is located at the center of the triangle.

☐ After

☐ Before

A diagram showing a pentagon with a dashed red boundary and a solid blue boundary. Inside the pentagon, there is a red dot and a blue dot, representing the centers of the two boundaries.

☐ After

86. For the image below, select whether the test shape (red dashed edges) comes after or before the reference shape (blue solid edges), as defined in the instructions above.

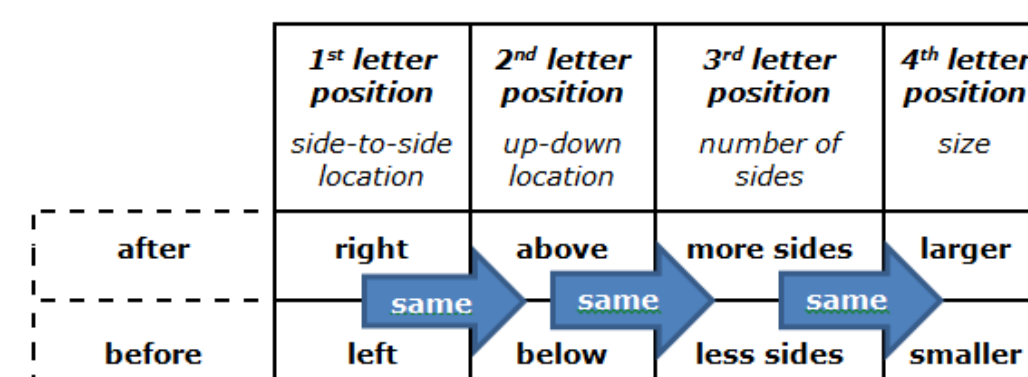

87. For the image below, select whether the test shape (red dashed edges) comes after or before the reference shape (blue solid edges), as defined in the instructions above.

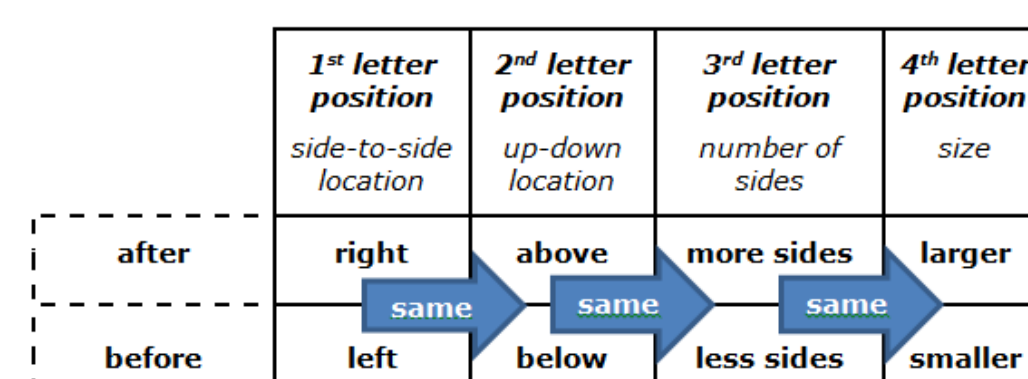

88. For the image below, select whether the test shape (red dashed edges) comes after or before the reference shape (blue solid edges), as defined in the instructions above.

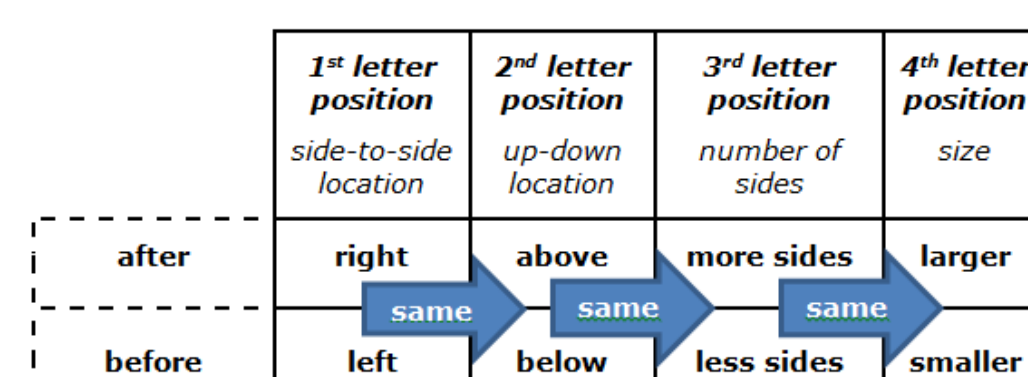

89. For the image below, select whether the test shape (red dashed edges) comes after or before the reference shape (blue solid edges), as defined in the instructions above.

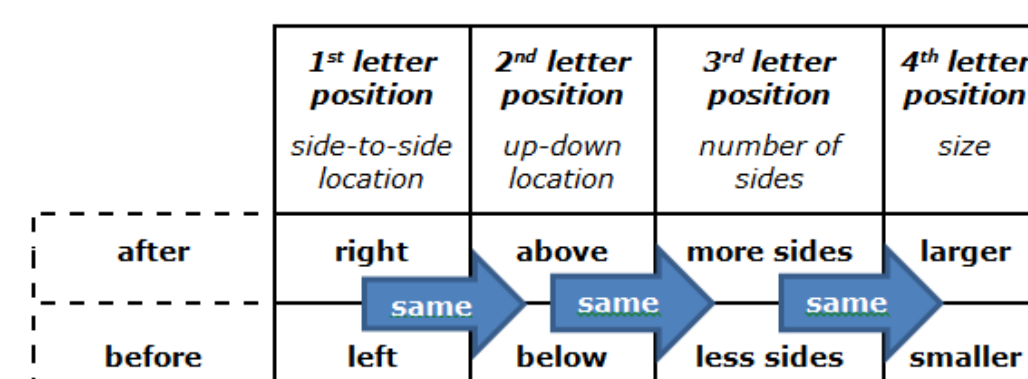

90. For the image below, select whether the test shape (red dashed edges) comes after or before the reference shape (blue solid edges), as defined in the instructions above.

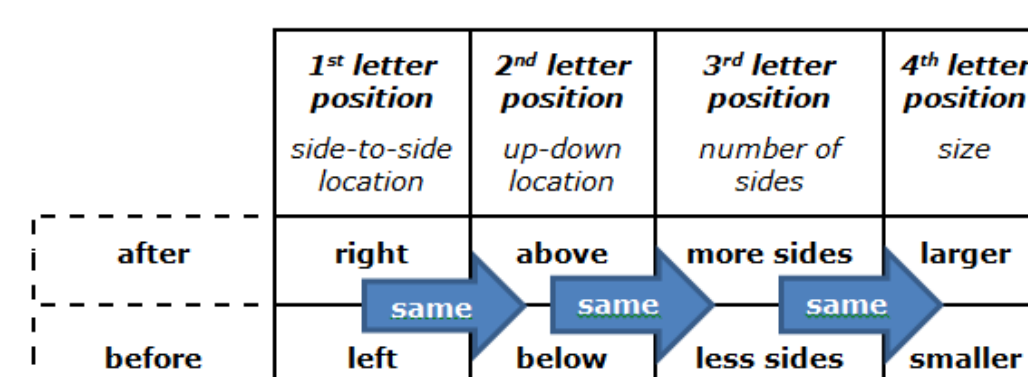

91. For the image below, select whether the test shape (red dashed edges) comes after or before the reference shape (blue solid edges), as defined in the instructions above.

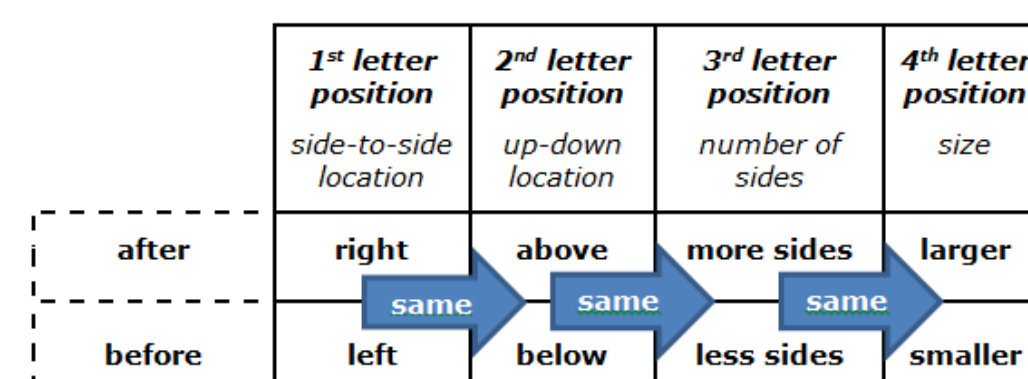

92. For the image below, select whether the test shape (red dashed edges) comes after or before the reference shape (blue solid edges), as defined in the instructions above.

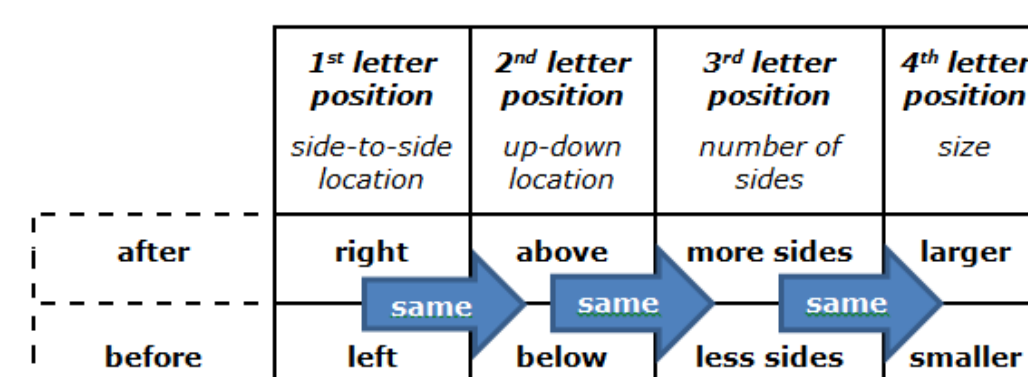

93. For the image below, select whether the test shape (red dashed edges) comes after or before the reference shape (blue solid edges), as defined in the instructions above.

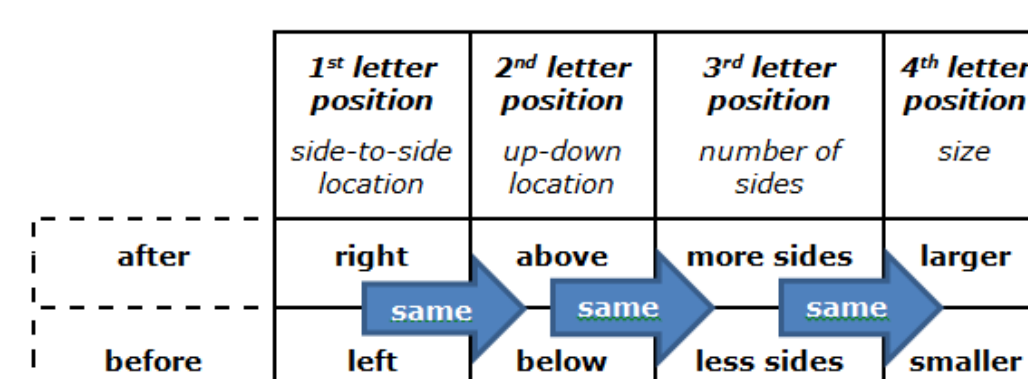

94. For the image below, select whether the test shape (red dashed edges) comes after or before the reference shape (blue solid edges), as defined in the instructions above.





☐ Before

103. For the image below, select whether the test shape (red dashed edges) comes after or before the reference shape (blue solid edges), as defined in the instructions above.

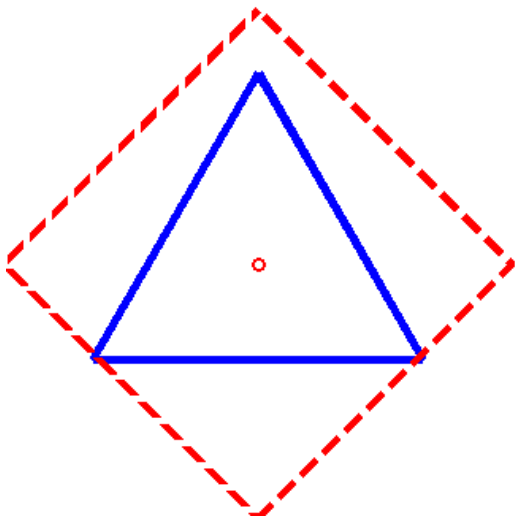

|        | 1 <sup>st</sup> letter<br>position<br>side-to-side<br>location | 2 <sup>nd</sup> letter<br>position<br>up-down<br>location | 3 <sup>rd</sup> letter<br>position<br>number of<br>sides | 4 <sup>th</sup> letter<br>position<br>size |
|--------|----------------------------------------------------------------|-----------------------------------------------------------|----------------------------------------------------------|--------------------------------------------|
| after  | right                                                          | above                                                     | more sides                                               | larger                                     |
| before | left                                                           | below                                                     | less sides                                               | smaller                                    |

☐ After  
☐ Before

104. For the image below, select whether the test shape (red dashed edges) comes after or before the reference shape (blue solid edges), as defined in the instructions above.

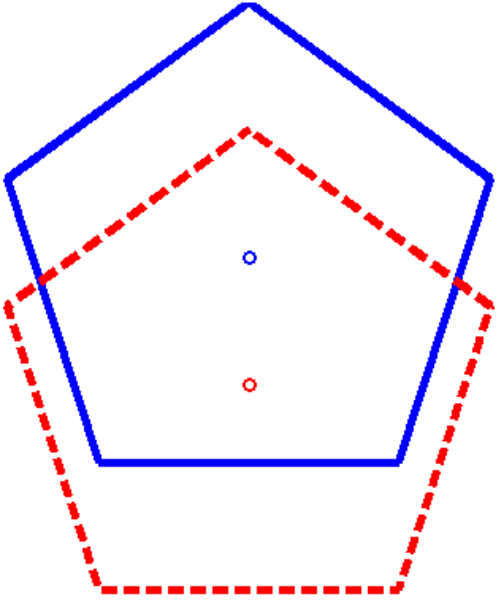

|        | 1 <sup>st</sup> letter<br>position<br>side-to-side<br>location | 2 <sup>nd</sup> letter<br>position<br>up-down<br>location | 3 <sup>rd</sup> letter<br>position<br>number of<br>sides | 4 <sup>th</sup> letter<br>position<br>size |
|--------|----------------------------------------------------------------|-----------------------------------------------------------|----------------------------------------------------------|--------------------------------------------|
| after  | right                                                          | above                                                     | more sides                                               | larger                                     |
| before | left                                                           | below                                                     | less sides                                               | smaller                                    |

☐ After  
☐ Before

105. For the image below, select whether the test shape (red dashed edges) comes after or before the reference shape (blue solid edges), as defined in the instructions above.

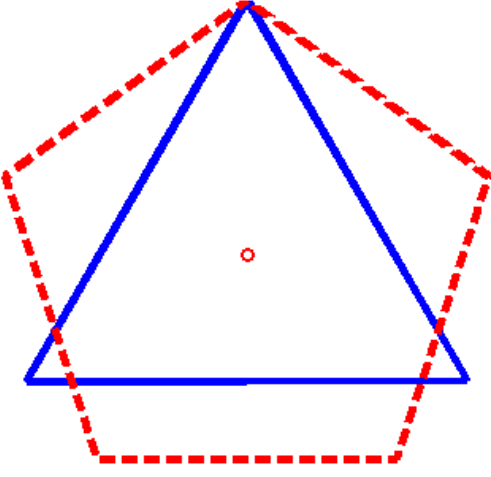

|        | 1 <sup>st</sup> letter<br>position<br>side-to-side<br>location | 2 <sup>nd</sup> letter<br>position<br>up-down<br>location | 3 <sup>rd</sup> letter<br>position<br>number of<br>sides | 4 <sup>th</sup> letter<br>position<br>size |
|--------|----------------------------------------------------------------|-----------------------------------------------------------|----------------------------------------------------------|--------------------------------------------|
| after  | right                                                          | above                                                     | more sides                                               | larger                                     |
| before | left                                                           | below                                                     | less sides                                               | smaller                                    |

☐ After  
☐ Before

106. For the image below, select whether the test shape (red dashed edges) comes after or before the reference shape (blue solid edges), as defined in the instructions above.

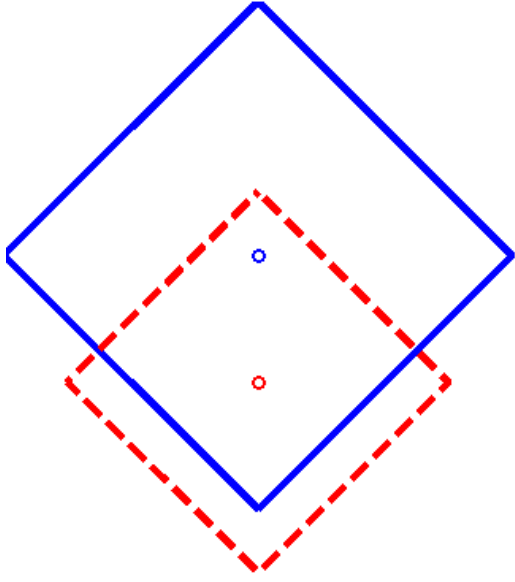

|        | 1 <sup>st</sup> letter<br>position<br>side-to-side<br>location | 2 <sup>nd</sup> letter<br>position<br>up-down<br>location | 3 <sup>rd</sup> letter<br>position<br>number of<br>sides | 4 <sup>th</sup> letter<br>position<br>size |
|--------|----------------------------------------------------------------|-----------------------------------------------------------|----------------------------------------------------------|--------------------------------------------|
| after  | right                                                          | above                                                     | more sides                                               | larger                                     |
| before | left                                                           | below                                                     | less sides                                               | smaller                                    |

☐ After  
☐ Before

107. For the image below, select whether the test shape (red dashed edges) comes after or before the reference shape (blue solid edges), as defined in the instructions above.

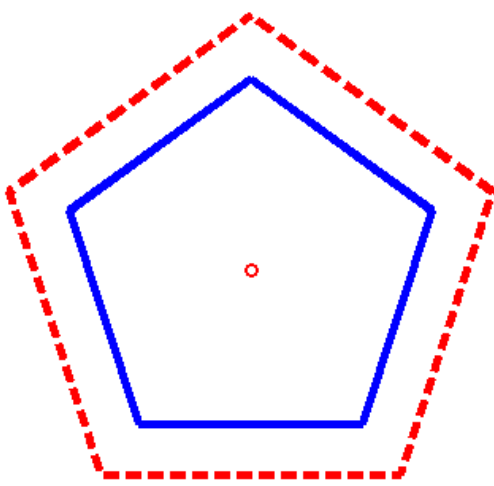

|        | 1 <sup>st</sup> letter<br>position<br>side-to-side<br>location | 2 <sup>nd</sup> letter<br>position<br>up-down<br>location | 3 <sup>rd</sup> letter<br>position<br>number of<br>sides | 4 <sup>th</sup> letter<br>position<br>size |
|--------|----------------------------------------------------------------|-----------------------------------------------------------|----------------------------------------------------------|--------------------------------------------|
| after  | right                                                          | above                                                     | more sides                                               | larger                                     |
| before | left                                                           | below                                                     | less sides                                               | smaller                                    |

☐ After  
☐ Before

108. For the image below, select whether the test shape (red dashed edges) comes after or before the reference shape (blue solid edges), as defined in the instructions above.

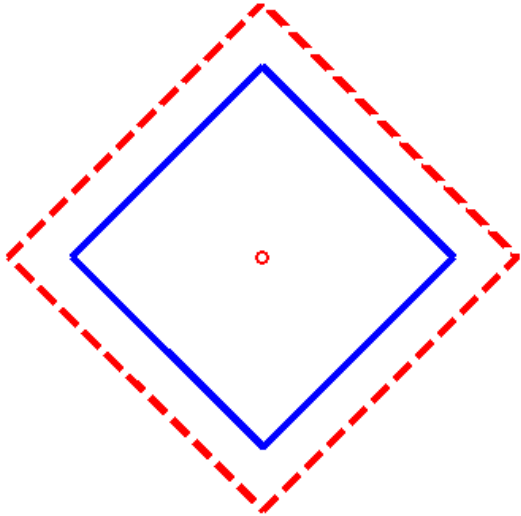

|        | 1 <sup>st</sup> letter<br>position<br>side-to-side<br>location | 2 <sup>nd</sup> letter<br>position<br>up-down<br>location | 3 <sup>rd</sup> letter<br>position<br>number of<br>sides | 4 <sup>th</sup> letter<br>position<br>size |
|--------|----------------------------------------------------------------|-----------------------------------------------------------|----------------------------------------------------------|--------------------------------------------|
| after  | right                                                          | above                                                     | more sides                                               | larger                                     |
| before | left                                                           | below                                                     | less sides                                               | smaller                                    |

☐ After  
☐ Before

109. For the image below, select whether the test shape (red dashed edges) comes after or before the reference shape (blue solid edges), as defined in the instructions above.

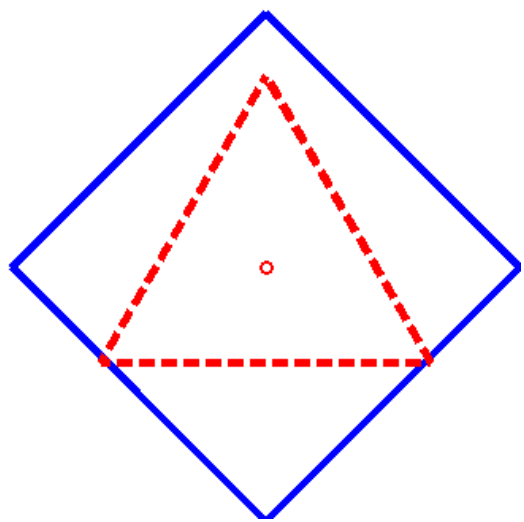

|        | 1 <sup>st</sup> letter<br>position<br>side-to-side<br>location | 2 <sup>nd</sup> letter<br>position<br>up-down<br>location | 3 <sup>rd</sup> letter<br>position<br>number of<br>sides | 4 <sup>th</sup> letter<br>position<br>size |
|--------|----------------------------------------------------------------|-----------------------------------------------------------|----------------------------------------------------------|--------------------------------------------|
| after  | right                                                          | above                                                     | more sides                                               | larger                                     |
| before | left                                                           | below                                                     | less sides                                               | smaller                                    |

☐ After  
☐ Before

110. For the image below, select whether the test shape (red dashed edges) comes after or before the reference shape (blue solid edges), as defined in the instructions above.

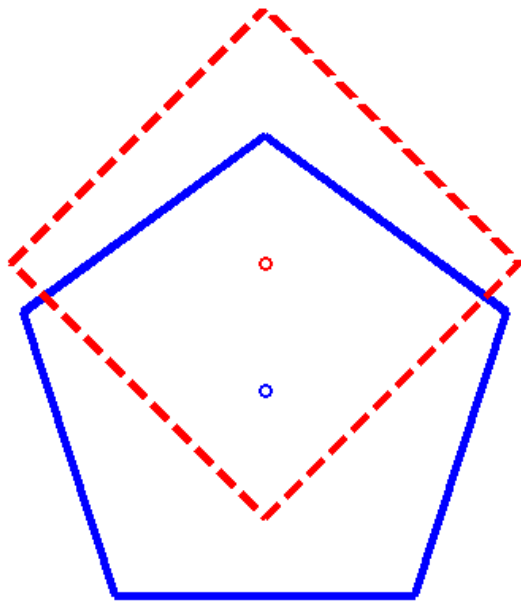

|        | 1 <sup>st</sup> letter<br>position<br>side-to-side<br>location | 2 <sup>nd</sup> letter<br>position<br>up-down<br>location | 3 <sup>rd</sup> letter<br>position<br>number of<br>sides | 4 <sup>th</sup> letter<br>position<br>size |
|--------|----------------------------------------------------------------|-----------------------------------------------------------|----------------------------------------------------------|--------------------------------------------|
| after  | right                                                          | above                                                     | more sides                                               | larger                                     |
| before | left                                                           | below                                                     | less sides                                               | smaller                                    |

☐ After  
☐ Before

111. For the image below, select whether the test shape (red dashed edges) comes after or before the reference shape (blue solid edges), as defined in the instructions above.



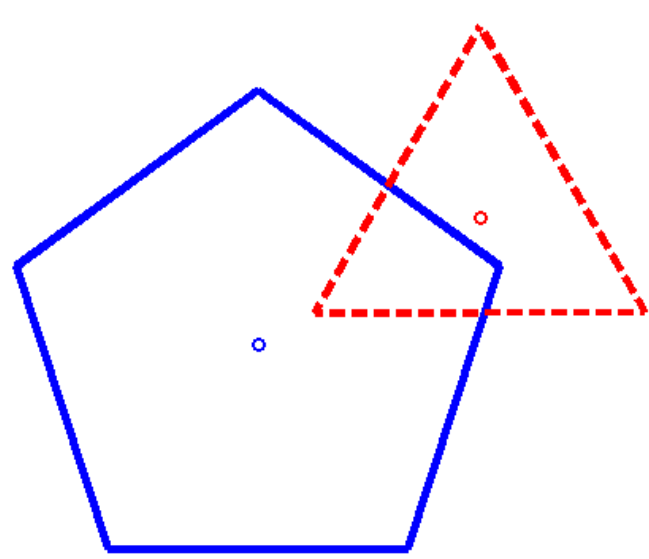

|        | 1 <sup>st</sup> letter position<br><i>side-to-side location</i> | 2 <sup>nd</sup> letter position<br><i>up-down location</i> | 3 <sup>rd</sup> letter position<br><i>number of sides</i> | 4 <sup>th</sup> letter position<br><i>size</i> |
|--------|-----------------------------------------------------------------|------------------------------------------------------------|-----------------------------------------------------------|------------------------------------------------|
| after  | right                                                           | above                                                      | more sides                                                | larger                                         |
| before | left                                                            | below                                                      | less sides                                                | smaller                                        |

☐ After

☐ Before

112. For the image below, select whether the test shape (red dashed edges) comes after or before the reference shape (blue solid edges), as defined in the instructions above.

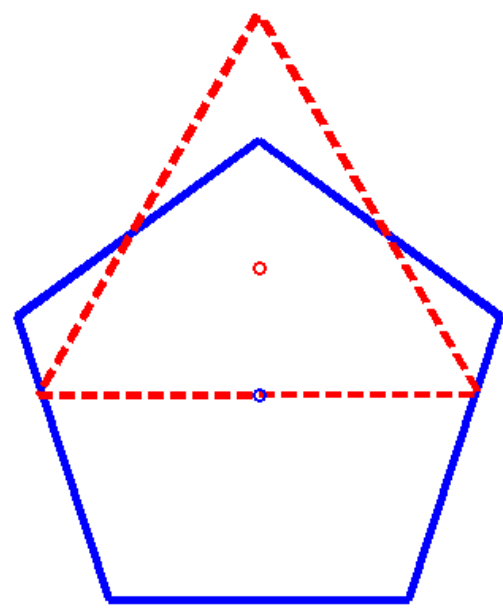

|        | 1 <sup>st</sup> letter position<br>side-to-side location | 2 <sup>nd</sup> letter position<br>up-down location | 3 <sup>rd</sup> letter position<br>number of sides | 4 <sup>th</sup> letter position<br>size |
|--------|----------------------------------------------------------|-----------------------------------------------------|----------------------------------------------------|-----------------------------------------|
| after  | right                                                    | above                                               | more sides                                         | larger                                  |
| before | left                                                     | below                                               | less sides                                         | smaller                                 |

☐ After

☐ Before

113. For the image below, select whether the test shape (red dashed edges) comes after or before the reference shape (blue solid edges), as defined in the instructions above.

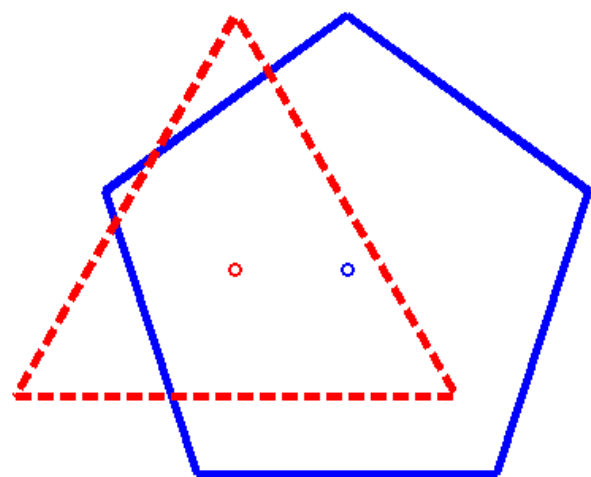

|        | 1 <sup>st</sup> letter position<br><i>side-to-side location</i> | 2 <sup>nd</sup> letter position<br><i>up-down location</i> | 3 <sup>rd</sup> letter position<br><i>number of sides</i> | 4 <sup>th</sup> letter position<br><i>size</i> |
|--------|-----------------------------------------------------------------|------------------------------------------------------------|-----------------------------------------------------------|------------------------------------------------|
| after  | right                                                           | above                                                      | more sides                                                | larger                                         |
| before | left                                                            | below                                                      | less sides                                                | smaller                                        |

☐ After

☐ Before

114. For the image below, select whether the test shape (red dashed edges) comes after or before the reference shape (blue solid edges), as defined in the instructions above.

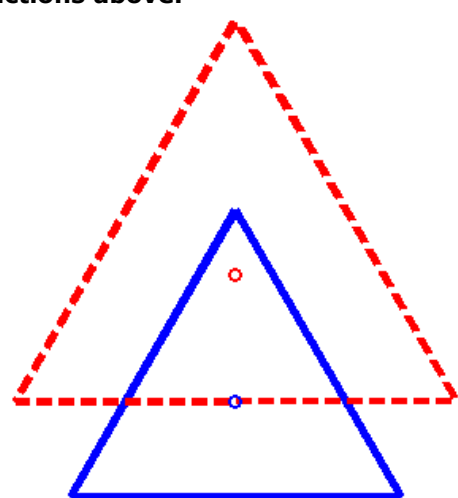

|        | 1 <sup>st</sup> letter position<br><i>side-to-side location</i> | 2 <sup>nd</sup> letter position<br><i>up-down location</i> | 3 <sup>rd</sup> letter position<br><i>number of sides</i> | 4 <sup>th</sup> letter position<br><i>size</i> |
|--------|-----------------------------------------------------------------|------------------------------------------------------------|-----------------------------------------------------------|------------------------------------------------|
| after  | right                                                           | above                                                      | more sides                                                | larger                                         |
| before | left                                                            | below                                                      | less sides                                                | smaller                                        |

☐ After

☐ Before

115. For the image below, select whether the test shape (red dashed edges) comes after or before the reference shape (blue solid edges), as defined in the instructions above.

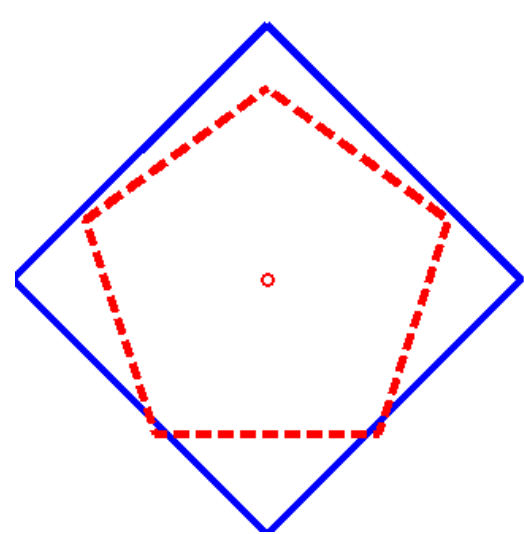

|        | 1 <sup>st</sup> letter position<br><i>side-to-side location</i> | 2 <sup>nd</sup> letter position<br><i>up-down location</i> | 3 <sup>rd</sup> letter position<br><i>number of sides</i> | 4 <sup>th</sup> letter position<br><i>size</i> |
|--------|-----------------------------------------------------------------|------------------------------------------------------------|-----------------------------------------------------------|------------------------------------------------|
| after  | right                                                           | above                                                      | more sides                                                | larger                                         |
| before | left                                                            | below                                                      | less sides                                                | smaller                                        |

☐ After

☐ Before

116. For the image below, select whether the test shape (red dashed edges) comes after or before the reference shape (blue solid edges), as defined in the instructions above.

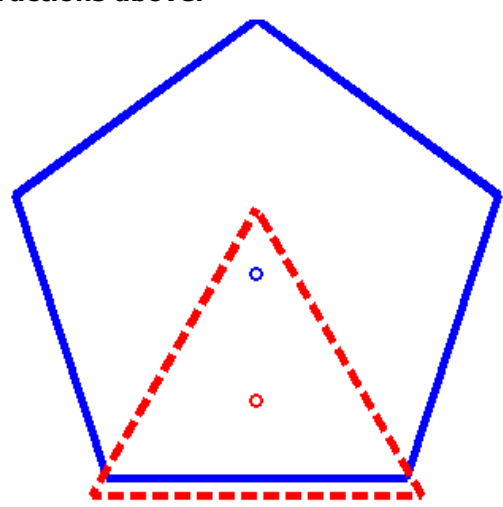

|        | 1 <sup>st</sup> letter position<br><i>side-to-side location</i> | 2 <sup>nd</sup> letter position<br><i>up-down location</i> | 3 <sup>rd</sup> letter position<br><i>number of sides</i> | 4 <sup>th</sup> letter position<br><i>size</i> |
|--------|-----------------------------------------------------------------|------------------------------------------------------------|-----------------------------------------------------------|------------------------------------------------|
| after  | right                                                           | above                                                      | more sides                                                | larger                                         |
| before | left                                                            | below                                                      | less sides                                                | smaller                                        |

☐ After

☐ Before

117. For the image below, select whether the test shape (red dashed edges) comes after or before the reference shape (blue solid edges), as defined in the instructions above.

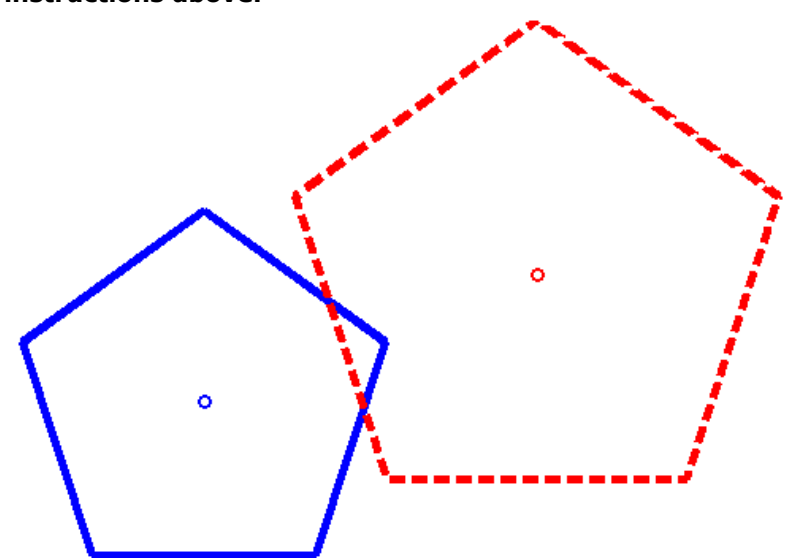

|        | 1 <sup>st</sup> letter position<br>side-to-side location | 2 <sup>nd</sup> letter position<br>up-down location | 3 <sup>rd</sup> letter position<br>number of sides | 4 <sup>th</sup> letter position<br>size |
|--------|----------------------------------------------------------|-----------------------------------------------------|----------------------------------------------------|-----------------------------------------|
| after  | right                                                    | above                                               | more sides                                         | larger                                  |
| before | left                                                     | below                                               | less sides                                         | smaller                                 |

☐ After

☐ Before

118. For the image below, select whether the test shape (red dashed edges) comes after or before the reference shape (blue solid edges), as defined in the instructions above.

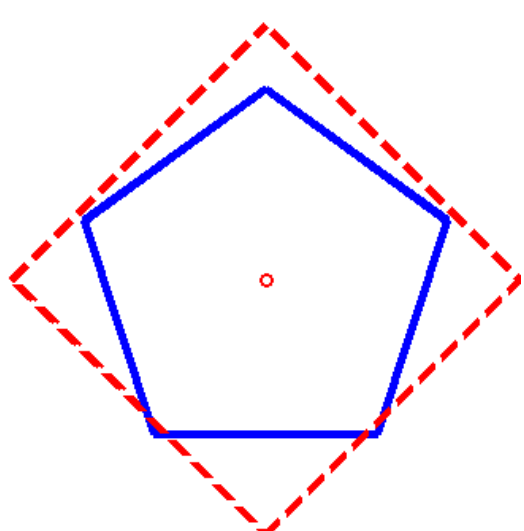

|        | 1 <sup>st</sup> letter position<br><i>side-to-side location</i> | 2 <sup>nd</sup> letter position<br><i>up-down location</i> | 3 <sup>rd</sup> letter position<br><i>number of sides</i> | 4 <sup>th</sup> letter position<br><i>size</i> |
|--------|-----------------------------------------------------------------|------------------------------------------------------------|-----------------------------------------------------------|------------------------------------------------|
| after  | right                                                           | above                                                      | more sides                                                | larger                                         |
| before | left                                                            | below                                                      | less sides                                                | smaller                                        |

☐ After

☐ Before

119. For the image below, select whether the test shape (red dashed edges) comes after or before the reference shape (blue solid edges), as defined in the instructions above.

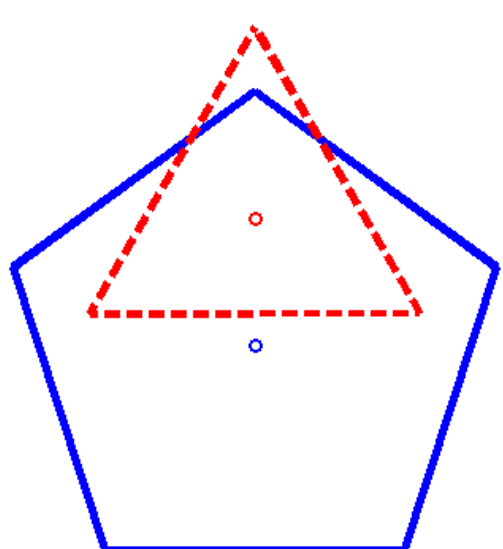

|        | 1 <sup>st</sup> letter position<br><i>side-to-side location</i> | 2 <sup>nd</sup> letter position<br><i>up-down location</i> | 3 <sup>rd</sup> letter position<br><i>number of sides</i> | 4 <sup>th</sup> letter position<br><i>size</i> |
|--------|-----------------------------------------------------------------|------------------------------------------------------------|-----------------------------------------------------------|------------------------------------------------|
| after  | right                                                           | above                                                      | more sides                                                | larger                                         |
| before | left                                                            | below                                                      | less sides                                                | smaller                                        |

☐ After

120. For the image below, select whether the test shape (red dashed edges) comes after or before the reference shape (blue solid edges), as defined in the instructions above.

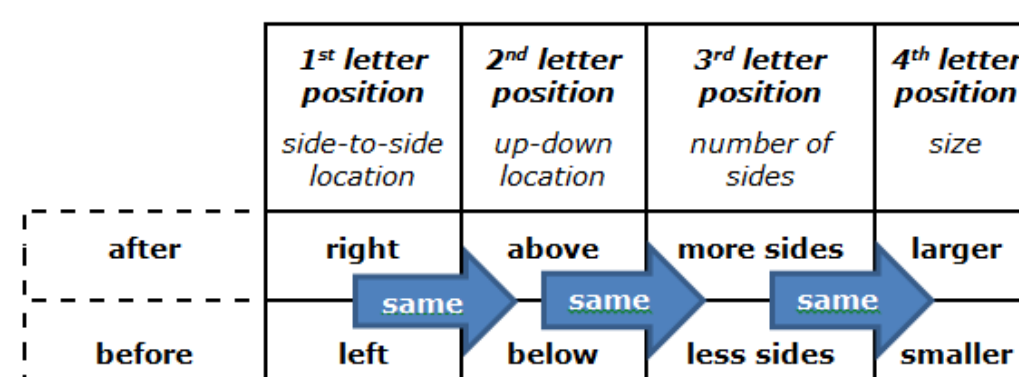

121. For the image below, select whether the test shape (red dashed edges) comes after or before the reference shape (blue solid edges), as defined in the instructions above.

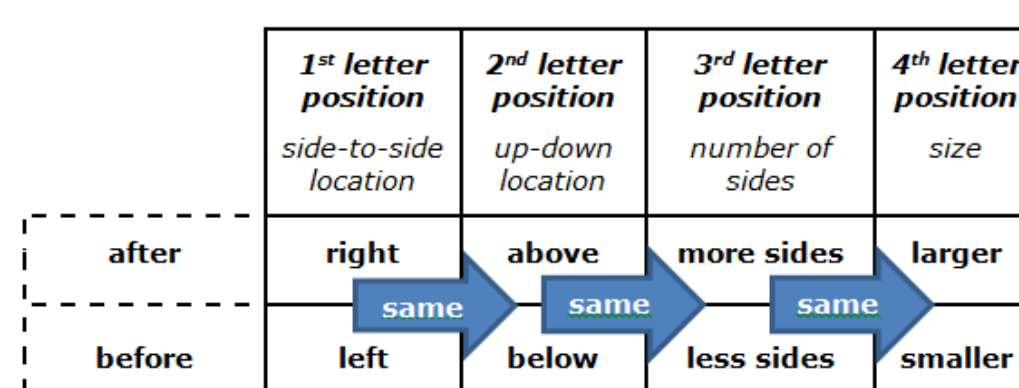

122. For the image below, select whether the test shape (red dashed edges) comes after or before the reference shape (blue solid edges), as defined in the instructions above.

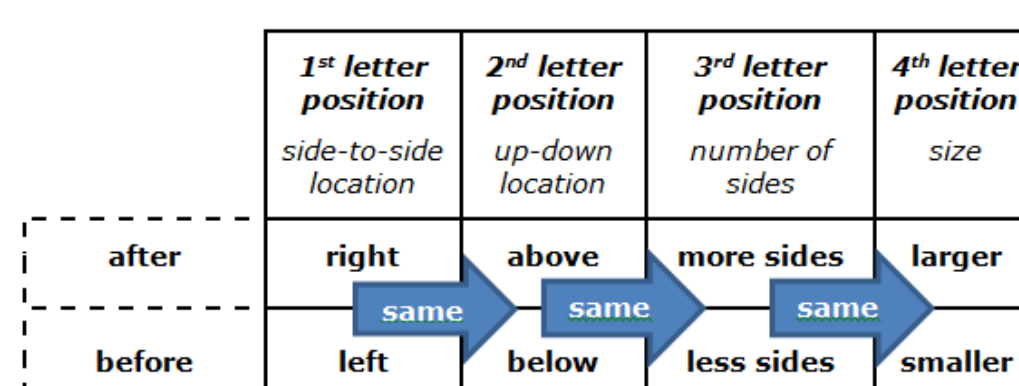

123. For the image below, select whether the test shape (red dashed edges) comes after or before the reference shape (blue solid edges), as defined in the instructions above.

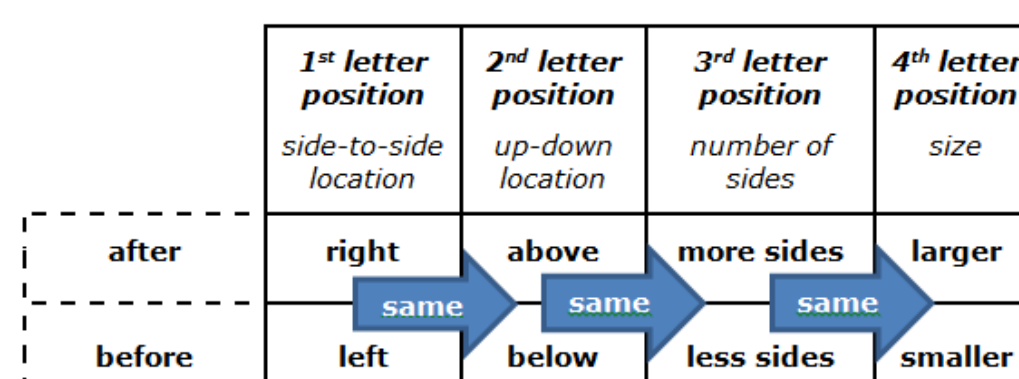

124. For the image below, select whether the test shape (red dashed edges) comes after or before the reference shape (blue solid edges), as defined in the instructions above.

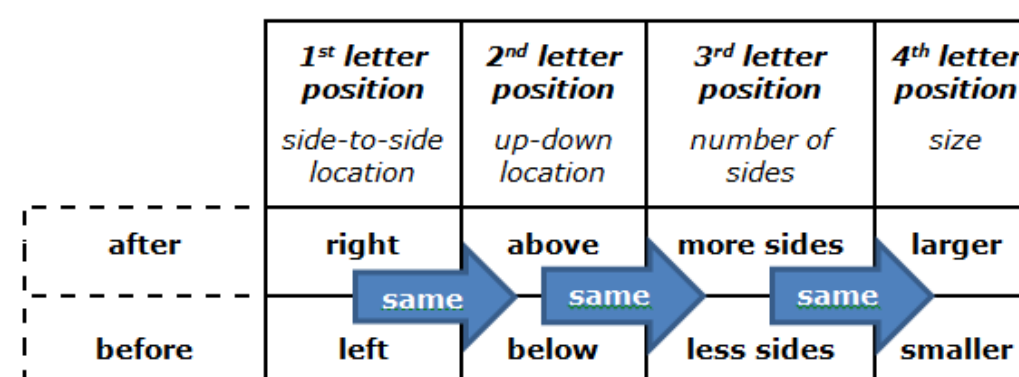

125. For the image below, select whether the test shape (red dashed edges) comes after or before the reference shape (blue solid edges), as defined in the instructions above.

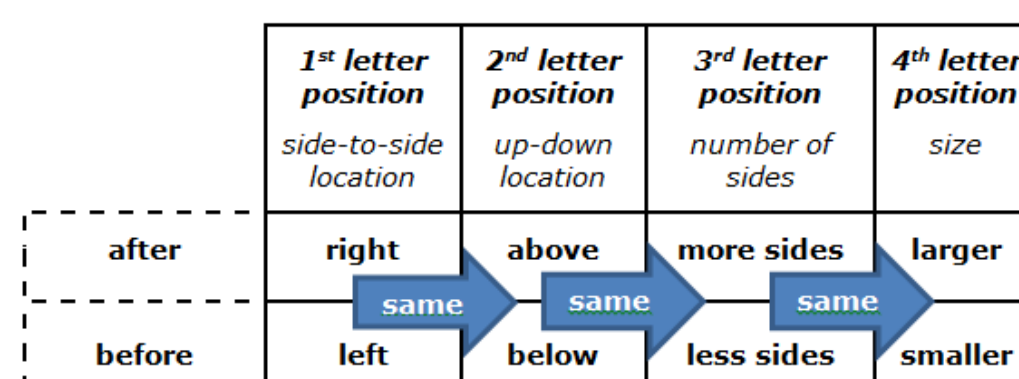

126. For the image below, select whether the test shape (red dashed edges) comes after or before the reference shape (blue solid edges), as defined in the instructions above.

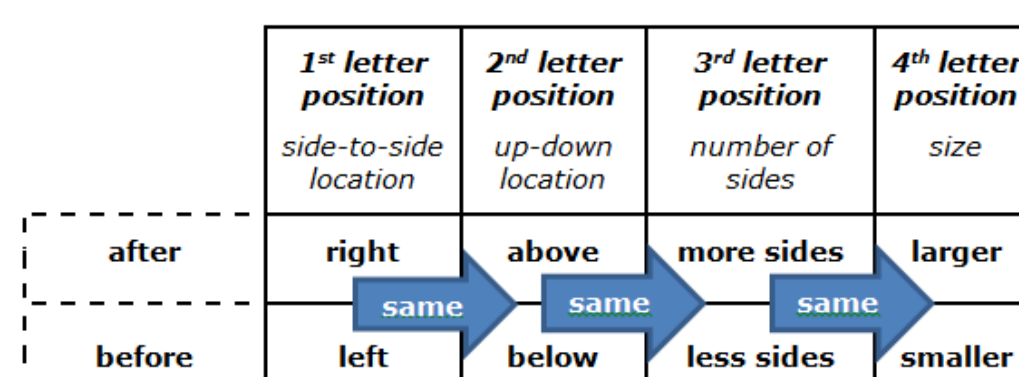

127. For the image below, select whether the test shape (red dashed edges) comes after or before the reference shape (blue solid edges), as defined in the instructions above.

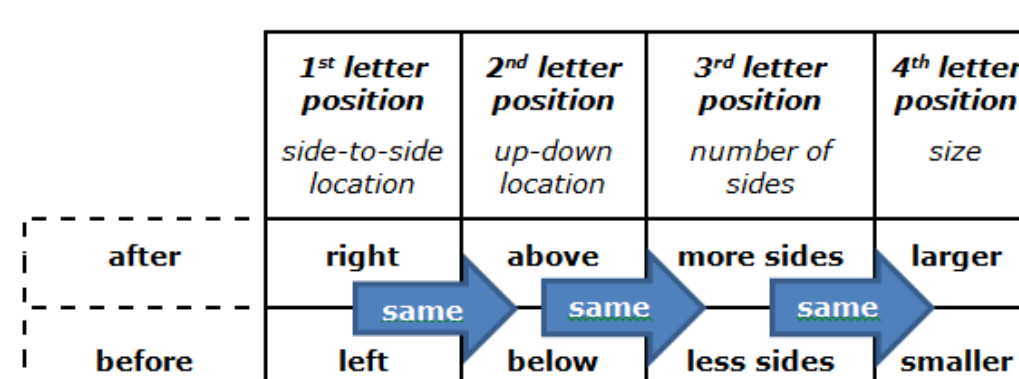

128. For the image below, select whether the test shape (red dashed edges) comes after or before the reference shape (blue solid edges), as defined in the instructions above.



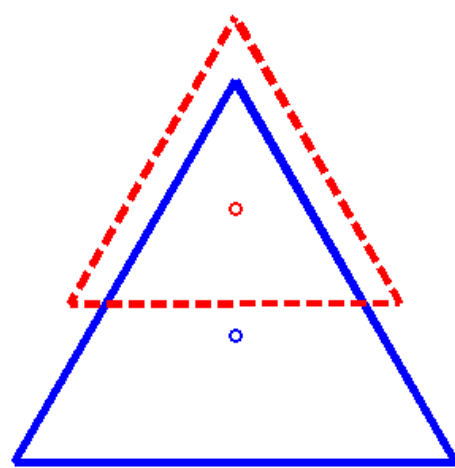

|        | 1 <sup>st</sup> letter position<br><i>side-to-side location</i> | 2 <sup>nd</sup> letter position<br><i>up-down location</i> | 3 <sup>rd</sup> letter position<br><i>number of sides</i> | 4 <sup>th</sup> letter position<br><i>size</i> |
|--------|-----------------------------------------------------------------|------------------------------------------------------------|-----------------------------------------------------------|------------------------------------------------|
| after  | right                                                           | above                                                      | more sides                                                | larger                                         |
| before | left                                                            | below                                                      | less sides                                                | smaller                                        |

☐ After

☐ Before

129. For the image below, select whether the test shape (red dashed edges) comes after or before the reference shape (blue solid edges), as defined in the instructions above.

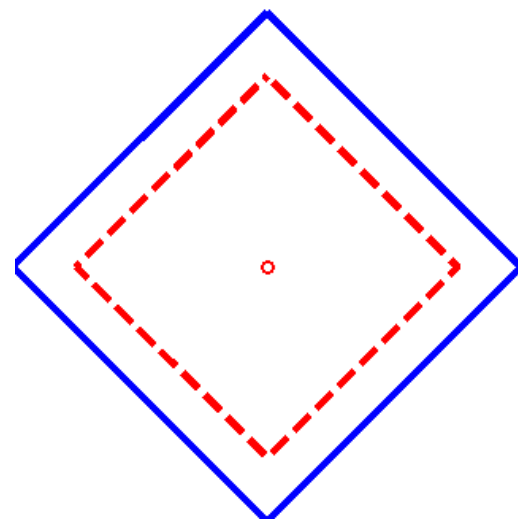

|        | 1 <sup>st</sup> letter position<br>side-to-side location | 2 <sup>nd</sup> letter position<br>up-down location | 3 <sup>rd</sup> letter position<br>number of sides | 4 <sup>th</sup> letter position<br>size |
|--------|----------------------------------------------------------|-----------------------------------------------------|----------------------------------------------------|-----------------------------------------|
| after  | right                                                    | above                                               | more sides                                         | larger                                  |
| before | left                                                     | below                                               | less sides                                         | smaller                                 |

☐ After

☐ Before

130. For the image below, select whether the test shape (red dashed edges) comes after or before the reference shape (blue solid edges), as defined in the instructions above.

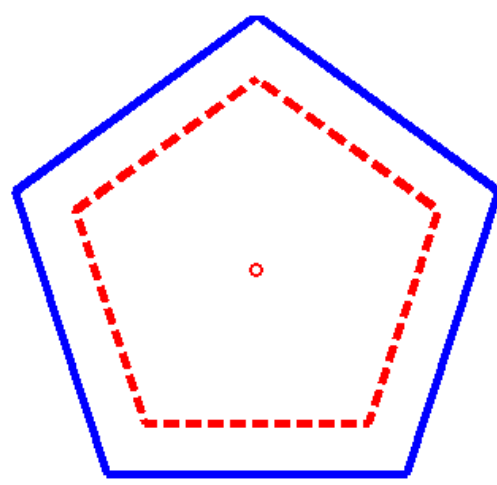

|        | 1 <sup>st</sup> letter position<br>side-to-side location | 2 <sup>nd</sup> letter position<br>up-down location | 3 <sup>rd</sup> letter position<br>number of sides | 4 <sup>th</sup> letter position<br>size |
|--------|----------------------------------------------------------|-----------------------------------------------------|----------------------------------------------------|-----------------------------------------|
| after  | right                                                    | above                                               | more sides                                         | larger                                  |
| before | left                                                     | below                                               | less sides                                         | smaller                                 |

☐ After

☐ Before

131. For the image below, select whether the test shape (red dashed edges) comes after or before the reference shape (blue solid edges), as defined in the instructions above.

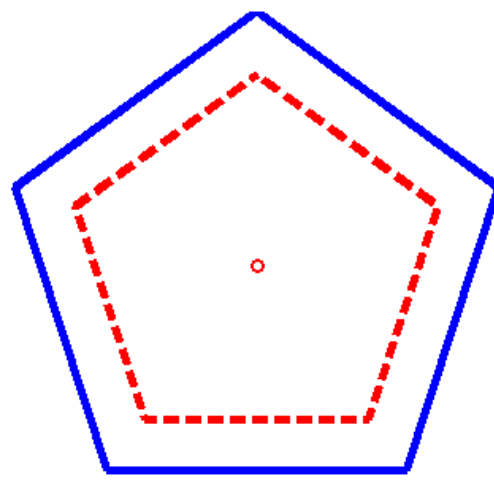

|        | 1 <sup>st</sup> letter position<br>side-to-side location | 2 <sup>nd</sup> letter position<br>up-down location | 3 <sup>rd</sup> letter position<br>number of sides | 4 <sup>th</sup> letter position<br>size |
|--------|----------------------------------------------------------|-----------------------------------------------------|----------------------------------------------------|-----------------------------------------|
| after  | right                                                    | above                                               | more sides                                         | larger                                  |
| before | left                                                     | below                                               | less sides                                         | smaller                                 |

☐ After

☐ Before

132. For the image below, select whether the test shape (red dashed edges) comes after or before the reference shape (blue solid edges), as defined in the instructions above.

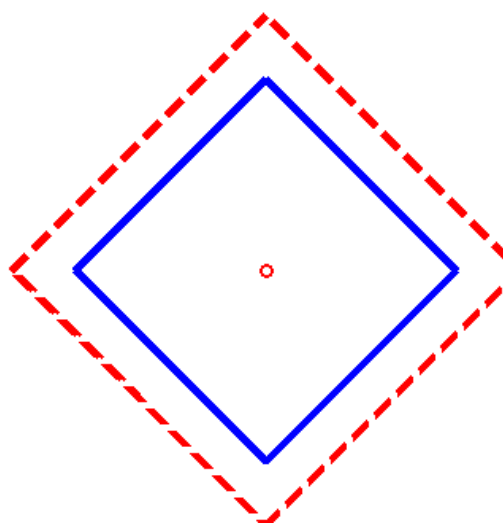

|        | 1 <sup>st</sup> letter position<br><i>side-to-side location</i> | 2 <sup>nd</sup> letter position<br><i>up-down location</i> | 3 <sup>rd</sup> letter position<br><i>number of sides</i> | 4 <sup>th</sup> letter position<br><i>size</i> |
|--------|-----------------------------------------------------------------|------------------------------------------------------------|-----------------------------------------------------------|------------------------------------------------|
| after  | right                                                           | above                                                      | more sides                                                | larger                                         |
| before | left                                                            | below                                                      | less sides                                                | smaller                                        |

☐ After

☐ Before

133. For the image below, select whether the test shape (red dashed edges) comes after or before the reference shape (blue solid edges), as defined in the instructions above.

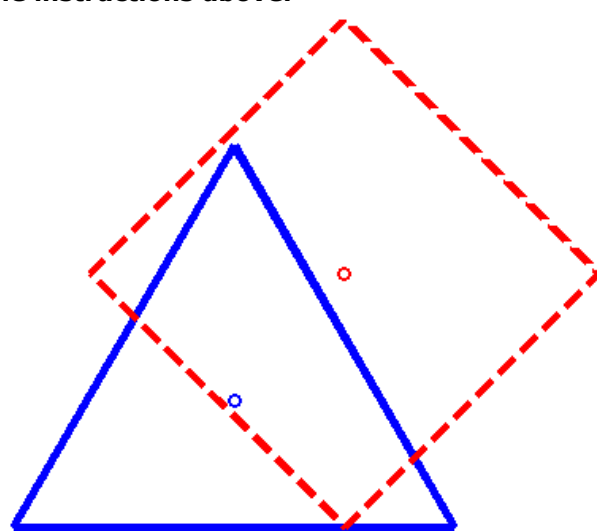

|        | 1 <sup>st</sup> letter position<br><i>side-to-side location</i> | 2 <sup>nd</sup> letter position<br><i>up-down location</i> | 3 <sup>rd</sup> letter position<br><i>number of sides</i> | 4 <sup>th</sup> letter position<br><i>size</i> |
|--------|-----------------------------------------------------------------|------------------------------------------------------------|-----------------------------------------------------------|------------------------------------------------|
| after  | right                                                           | above                                                      | more sides                                                | larger                                         |
| before | left                                                            | below                                                      | less sides                                                | smaller                                        |

☐ After

☐ Before

134. For the image below, select whether the test shape (red dashed edges) comes after or before the reference shape (blue solid edges), as defined in the instructions above.

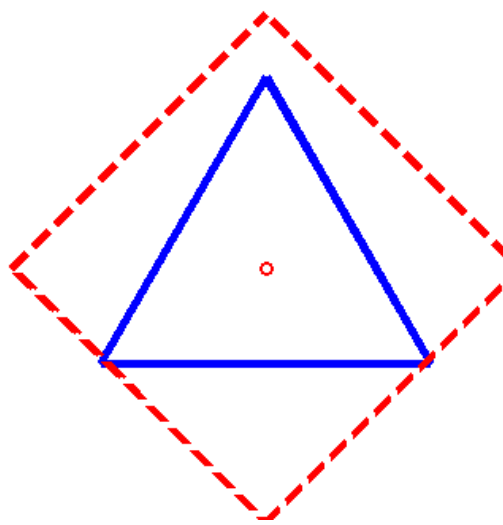

|        | 1 <sup>st</sup> letter position<br>side-to-side location | 2 <sup>nd</sup> letter position<br>up-down location | 3 <sup>rd</sup> letter position<br>number of sides | 4 <sup>th</sup> letter position<br>size |
|--------|----------------------------------------------------------|-----------------------------------------------------|----------------------------------------------------|-----------------------------------------|
| after  | right                                                    | above                                               | more sides                                         | larger                                  |
| before | left                                                     | below                                               | less sides                                         | smaller                                 |

☐ After

☐ Before

135. For the image below, select whether the test shape (red dashed edges) comes after or before the reference shape (blue solid edges), as defined in the instructions above.

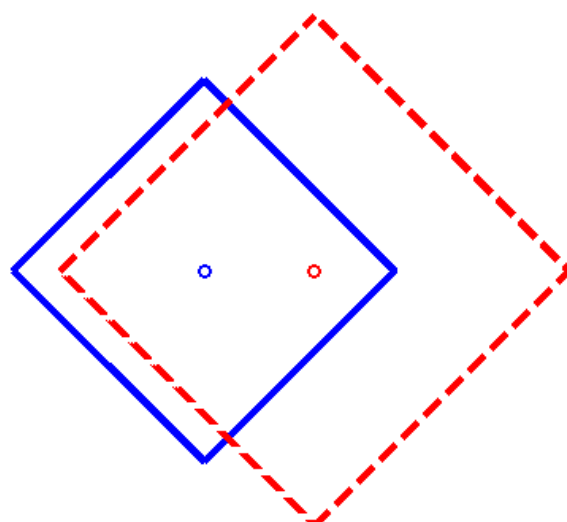

|        | 1 <sup>st</sup> letter position<br><i>side-to-side location</i> | 2 <sup>nd</sup> letter position<br><i>up-down location</i> | 3 <sup>rd</sup> letter position<br><i>number of sides</i> | 4 <sup>th</sup> letter position<br><i>size</i> |
|--------|-----------------------------------------------------------------|------------------------------------------------------------|-----------------------------------------------------------|------------------------------------------------|
| after  | right                                                           | above                                                      | more sides                                                | larger                                         |
| before | left                                                            | below                                                      | less sides                                                | smaller                                        |

☐ After

☐ Before

136. For the image below, select whether the test shape (red dashed edges) comes after or before the reference shape (blue solid edges), as defined in the instructions above.

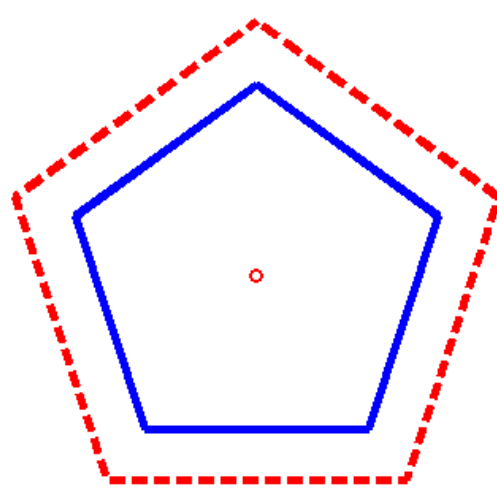

|        | 1 <sup>st</sup> letter position<br><i>side-to-side location</i> | 2 <sup>nd</sup> letter position<br><i>up-down location</i> | 3 <sup>rd</sup> letter position<br><i>number of sides</i> | 4 <sup>th</sup> letter position<br><i>size</i> |
|--------|-----------------------------------------------------------------|------------------------------------------------------------|-----------------------------------------------------------|------------------------------------------------|
| after  | right                                                           | above                                                      | more sides                                                | larger                                         |
| before | left                                                            | below                                                      | less sides                                                | smaller                                        |

☐ After

137. For the image below, select whether the test shape (red dashed edges) comes after or before the reference shape (blue solid edges), as defined in the instructions above.

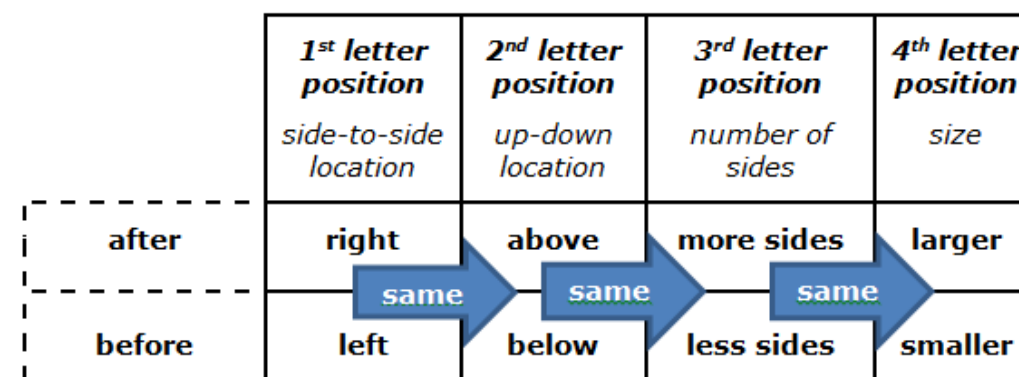

138. For the image below, select whether the test shape (red dashed edges) comes after or before the reference shape (blue solid edges), as defined in the instructions above.

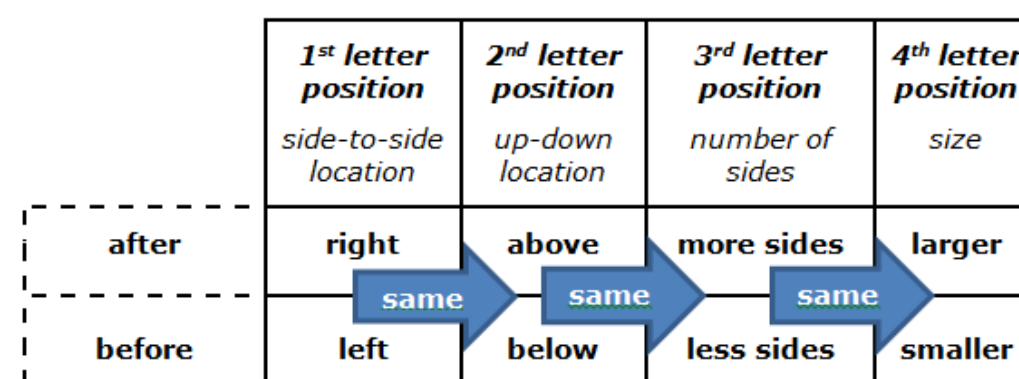

139. For the image below, select whether the test shape (red dashed edges) comes after or before the reference shape (blue solid edges), as defined in the instructions above.

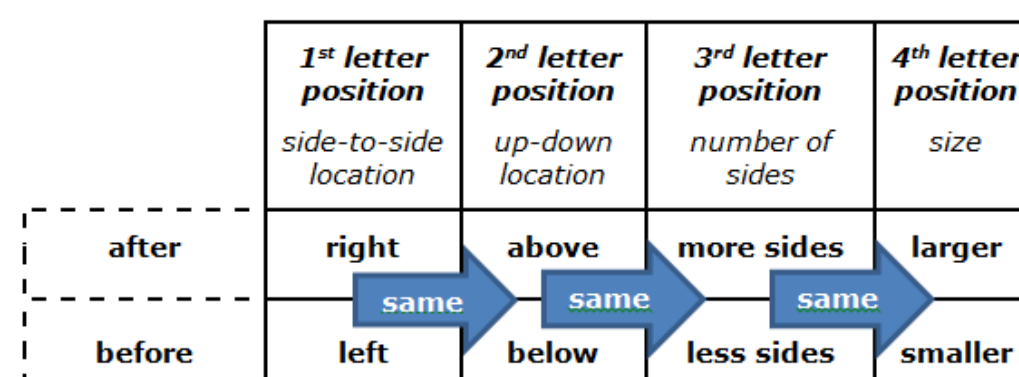

140. For the image below, select whether the test shape (red dashed edges) comes after or before the reference shape (blue solid edges), as defined in the instructions above.

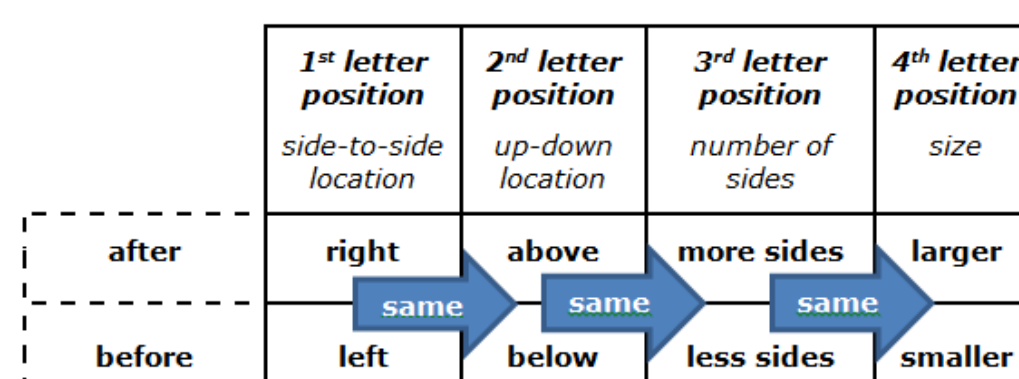

141. For the image below, select whether the test shape (red dashed edges) comes after or before the reference shape (blue solid edges), as defined in the instructions above

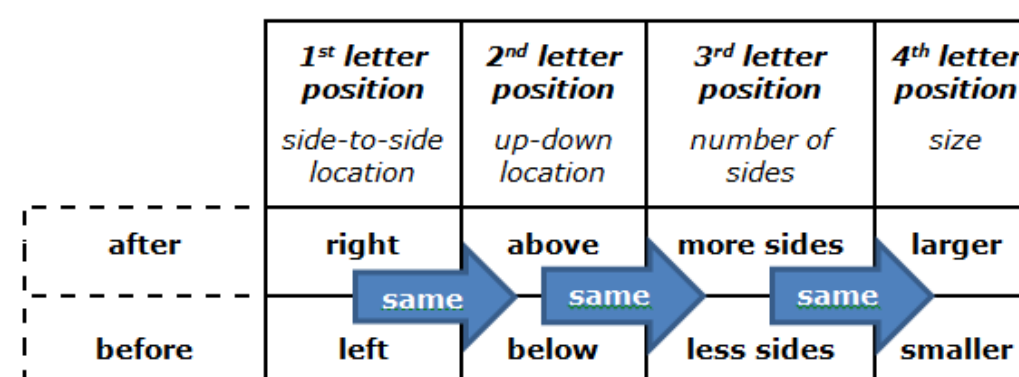

142. For the image below, select whether the test shape (red dashed edges) comes after or before the reference shape (blue solid edges), as defined in the instructions above.

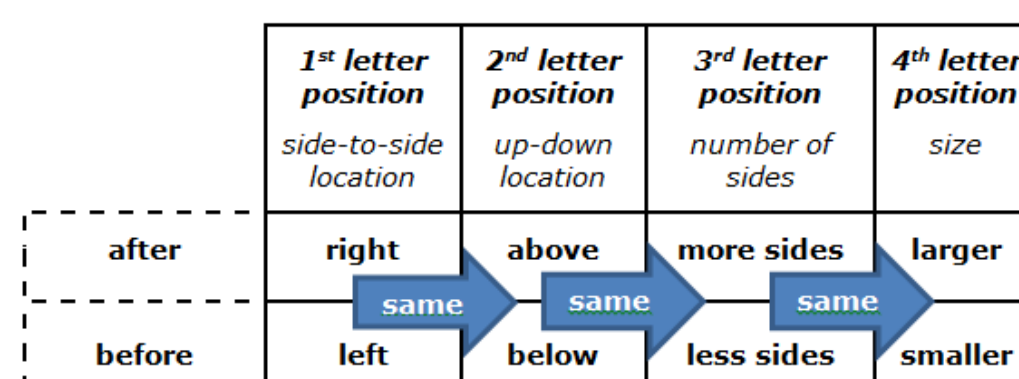

143. For the image below, select whether the test shape (red dashed edges) comes after or before the reference shape (blue solid edges), as defined in the instructions above

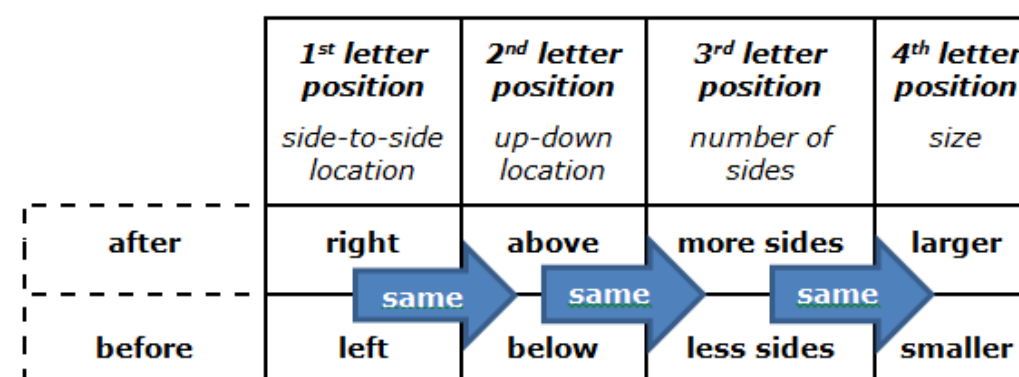

144. For the image below, select whether the test shape (red dashed edges) comes after or before the reference shape (blue solid edges), as defined in the instructions above.

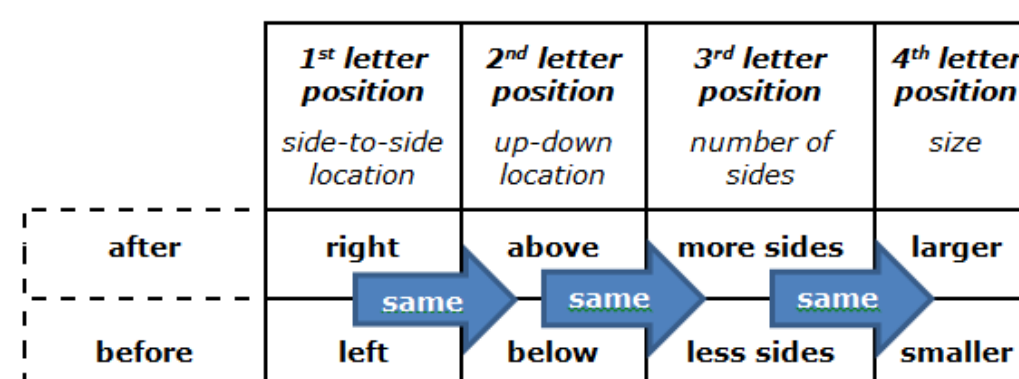

145. For the image below, select whether the test shape (red dashed edges) comes after or before the reference shape (blue solid edges), as defined in the instructions above.



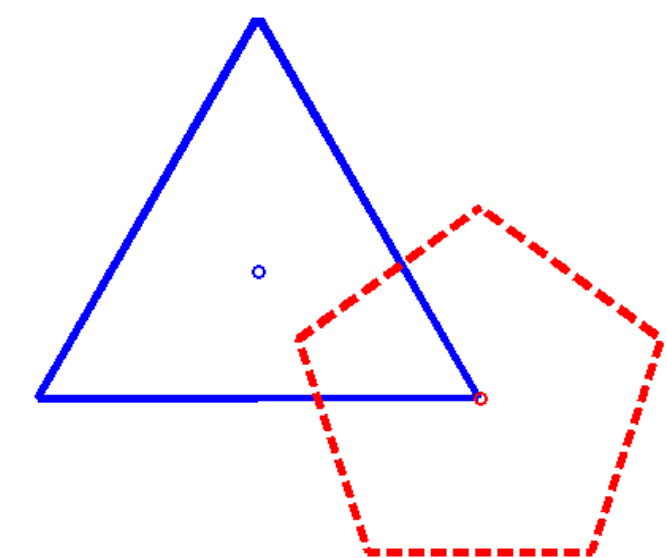

|        | 1 <sup>st</sup> letter<br>position<br>side-to-side<br>location | 2 <sup>nd</sup> letter<br>position<br>up-down<br>location | 3 <sup>rd</sup> letter<br>position<br>number of<br>sides | 4 <sup>th</sup> letter<br>position<br>size |
|--------|----------------------------------------------------------------|-----------------------------------------------------------|----------------------------------------------------------|--------------------------------------------|
| after  | right                                                          | above                                                     | more sides                                               | larger                                     |
|        | same                                                           | same                                                      | same                                                     |                                            |
| before | left                                                           | below                                                     | less sides                                               | smaller                                    |

☐ After  
☐ Before

146. For the image below, select whether the test shape (red dashed edges) comes after or before the reference shape (blue solid edges), as defined in the instructions above.

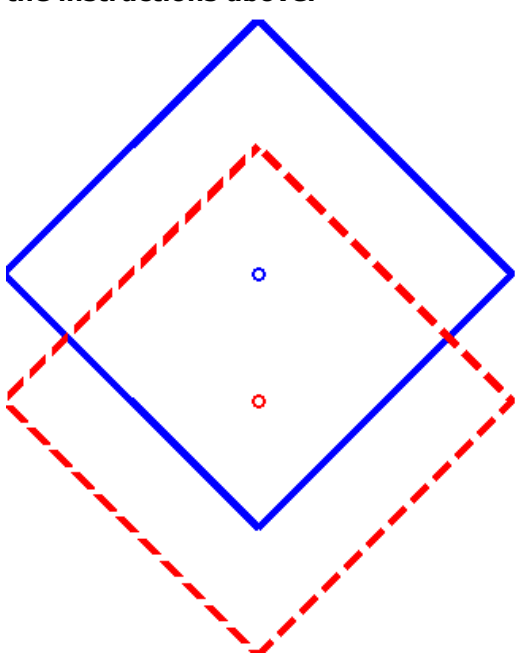

|        | 1 <sup>st</sup> letter<br>position<br>side-to-side<br>location | 2 <sup>nd</sup> letter<br>position<br>up-down<br>location | 3 <sup>rd</sup> letter<br>position<br>number of<br>sides | 4 <sup>th</sup> letter<br>position<br>size |
|--------|----------------------------------------------------------------|-----------------------------------------------------------|----------------------------------------------------------|--------------------------------------------|
| after  | right                                                          | above                                                     | more sides                                               | larger                                     |
|        | same                                                           | same                                                      | same                                                     |                                            |
| before | left                                                           | below                                                     | less sides                                               | smaller                                    |

☐ After  
☐ Before

147. For the image below, select whether the test shape (red dashed edges) comes after or before the reference shape (blue solid edges), as defined in the instructions above.

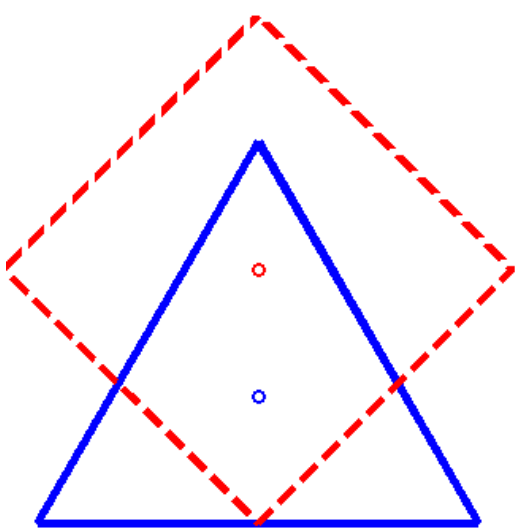

|        | 1 <sup>st</sup> letter<br>position<br>side-to-side<br>location | 2 <sup>nd</sup> letter<br>position<br>up-down<br>location | 3 <sup>rd</sup> letter<br>position<br>number of<br>sides | 4 <sup>th</sup> letter<br>position<br>size |
|--------|----------------------------------------------------------------|-----------------------------------------------------------|----------------------------------------------------------|--------------------------------------------|
| after  | right                                                          | above                                                     | more sides                                               | larger                                     |
|        | same                                                           | same                                                      | same                                                     |                                            |
| before | left                                                           | below                                                     | less sides                                               | smaller                                    |

☐ After  
☐ Before

148. For the image below, select whether the test shape (red dashed edges) comes after or before the reference shape (blue solid edges), as defined in the instructions above.

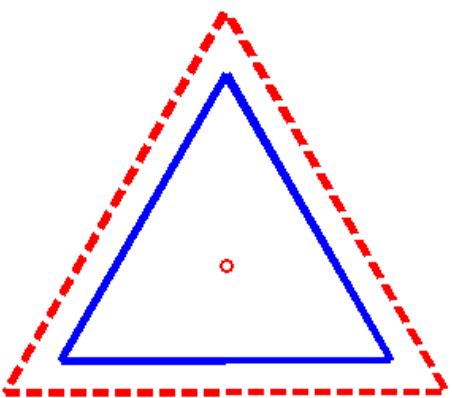

|        | 1 <sup>st</sup> letter<br>position<br>side-to-side<br>location | 2 <sup>nd</sup> letter<br>position<br>up-down<br>location | 3 <sup>rd</sup> letter<br>position<br>number of<br>sides | 4 <sup>th</sup> letter<br>position<br>size |
|--------|----------------------------------------------------------------|-----------------------------------------------------------|----------------------------------------------------------|--------------------------------------------|
| after  | right                                                          | above                                                     | more sides                                               | larger                                     |
|        | same                                                           | same                                                      | same                                                     |                                            |
| before | left                                                           | below                                                     | less sides                                               | smaller                                    |

☐ After  
☐ Before

149. For the image below, select whether the test shape (red dashed edges) comes after or before the reference shape (blue solid edges), as defined in the instructions above.

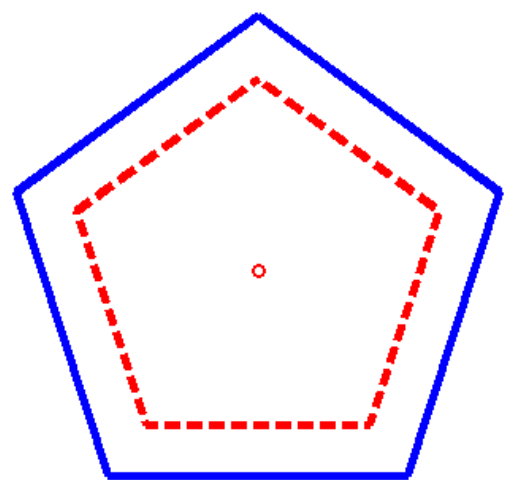

|        | 1 <sup>st</sup> letter<br>position<br>side-to-side<br>location | 2 <sup>nd</sup> letter<br>position<br>up-down<br>location | 3 <sup>rd</sup> letter<br>position<br>number of<br>sides | 4 <sup>th</sup> letter<br>position<br>size |
|--------|----------------------------------------------------------------|-----------------------------------------------------------|----------------------------------------------------------|--------------------------------------------|
| after  | right                                                          | above                                                     | more sides                                               | larger                                     |
|        | same                                                           | same                                                      | same                                                     |                                            |
| before | left                                                           | below                                                     | less sides                                               | smaller                                    |

☐ After  
☐ Before

150. For the image below, select whether the test shape (red dashed edges) comes after or before the reference shape (blue solid edges), as defined in the instructions above.

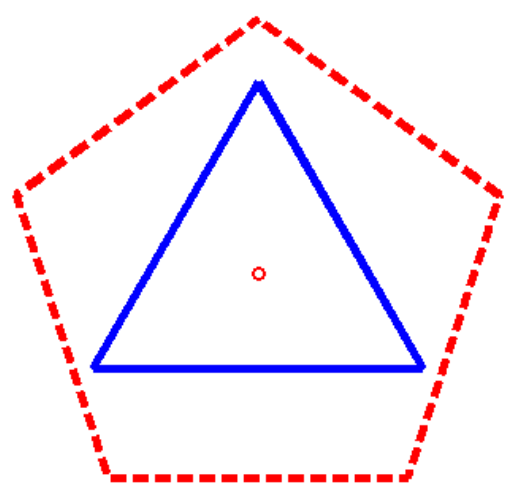

|        | 1 <sup>st</sup> letter<br>position<br>side-to-side<br>location | 2 <sup>nd</sup> letter<br>position<br>up-down<br>location | 3 <sup>rd</sup> letter<br>position<br>number of<br>sides | 4 <sup>th</sup> letter<br>position<br>size |
|--------|----------------------------------------------------------------|-----------------------------------------------------------|----------------------------------------------------------|--------------------------------------------|
| after  | right                                                          | above                                                     | more sides                                               | larger                                     |
|        | same                                                           | same                                                      | same                                                     |                                            |
| before | left                                                           | below                                                     | less sides                                               | smaller                                    |

☐ After  
☐ Before

\*\*\*After you have completed **EVERY** question in this HIT, click the submit button below. Note that incomplete HITs will **NOT** be approved and can **NOT** be resubmitted\*\*\*
